# Supplementary material for: The Active Asteroids Citizen Science Program: Overview and First Results
Source: arXiv:2403.09768 source file (2024-03-14)
Supplement: Supplementary file 1 [file AppendixCitSci.tex]

\section{Citizen Science Supplemental Material}

\label{sec:citSciSupp}

\subsection{Tutorial Images}

\label{sec:tutorialSupplemental}

\begin{figure}

    \centering

    \begin{tabular}{cccc}

    % \hline\\

        \includegraphics[width=0.22\linewidth]{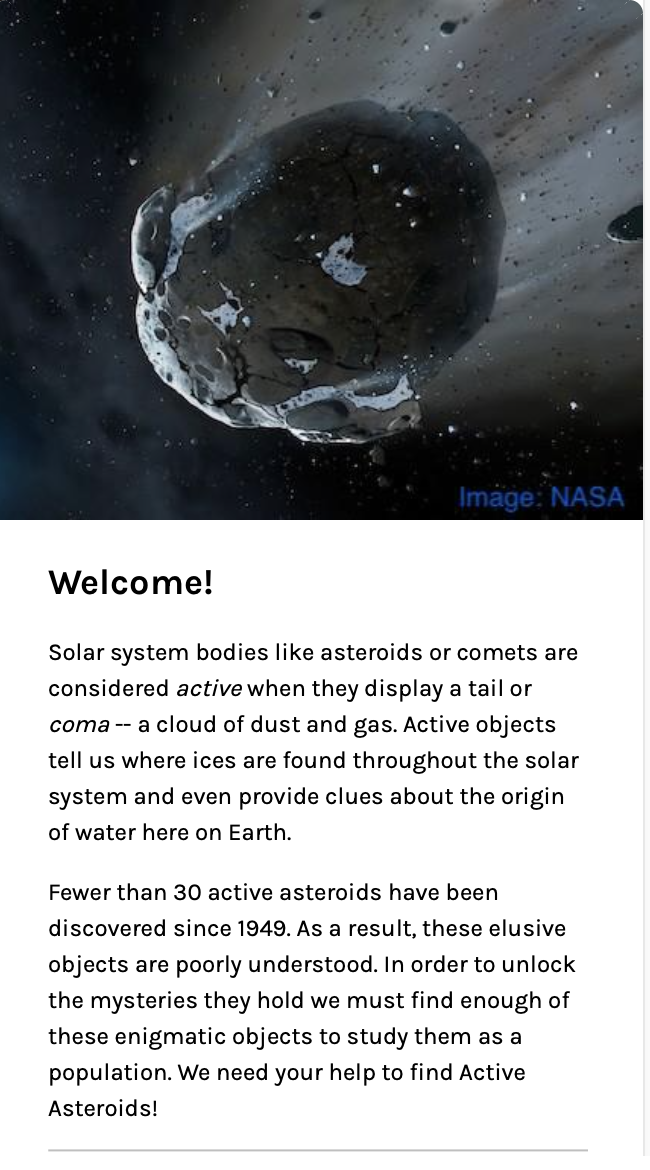} & \includegraphics[width=0.22\linewidth]{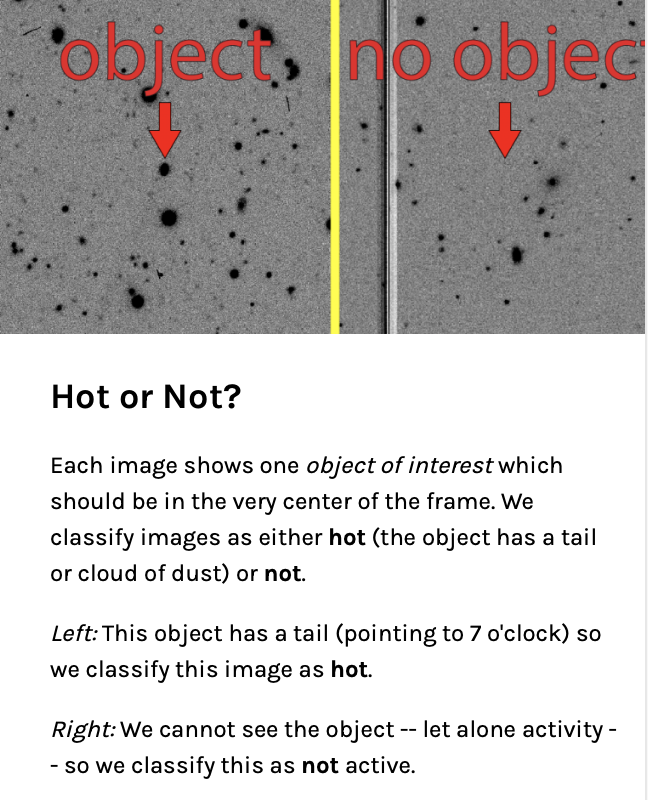} & \includegraphics[width=0.22\linewidth]{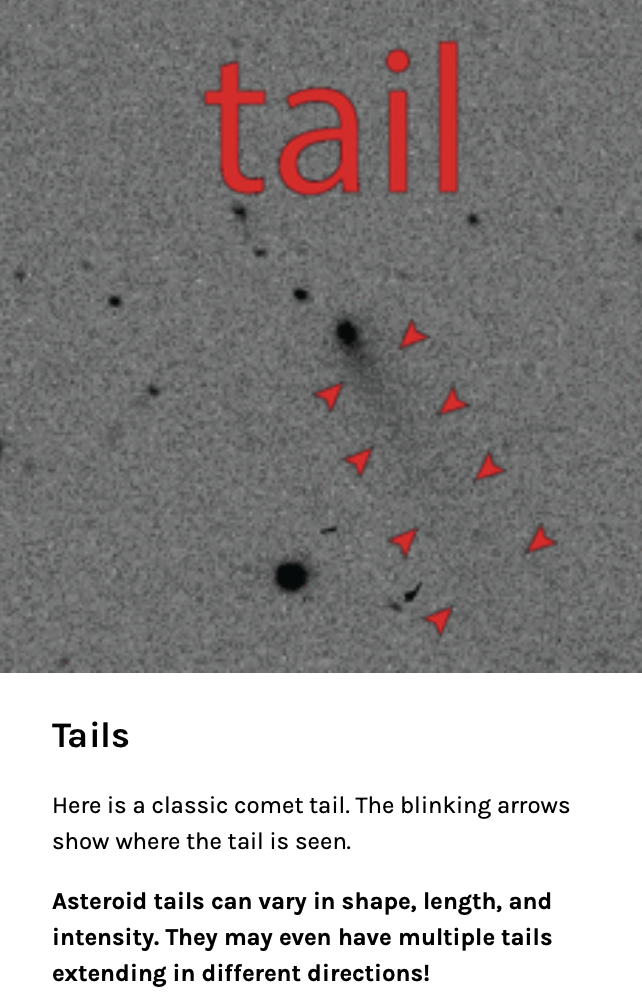} & \includegraphics[width=0.22\linewidth]{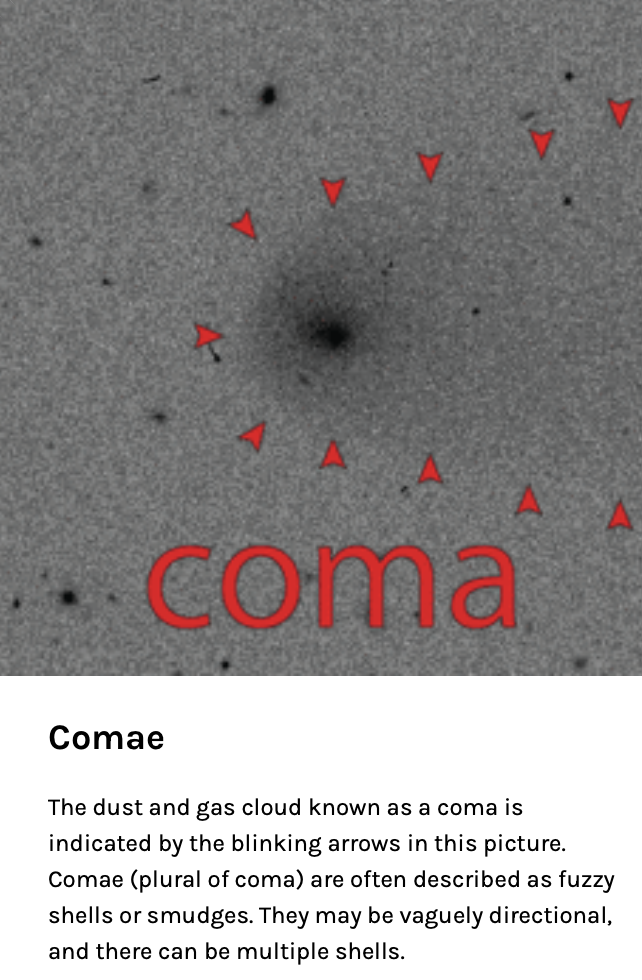}\\

        (1) & (2) & (3) & (4) \\

        % \hline\\

        \\

        \includegraphics[width=0.22\linewidth]{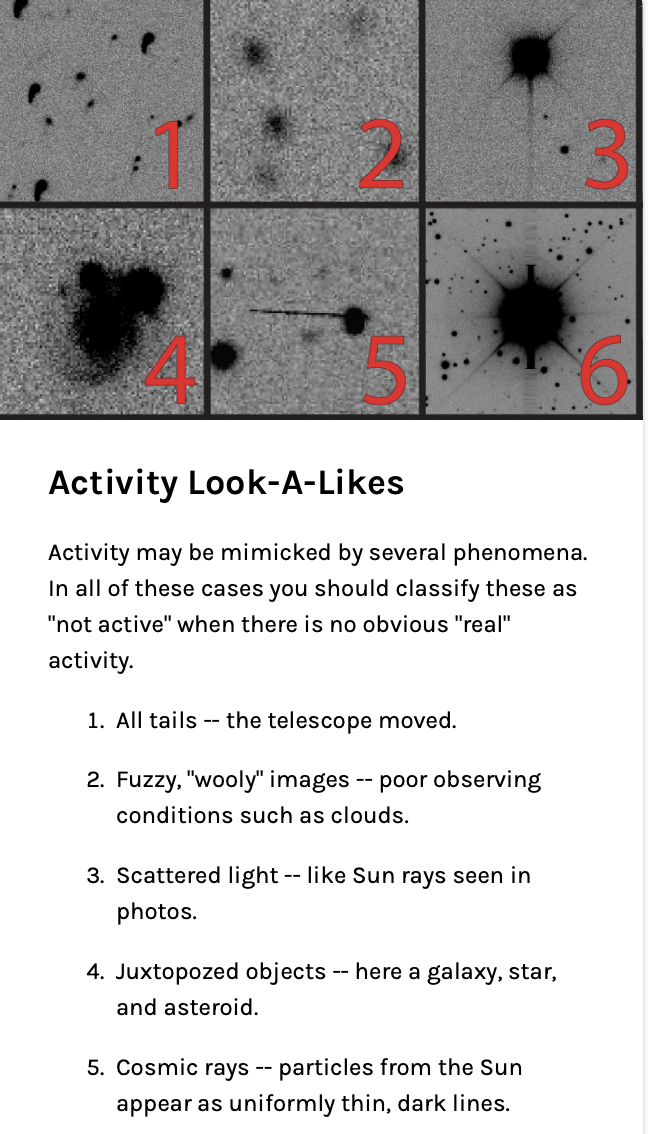} & \includegraphics[width=0.22\linewidth]{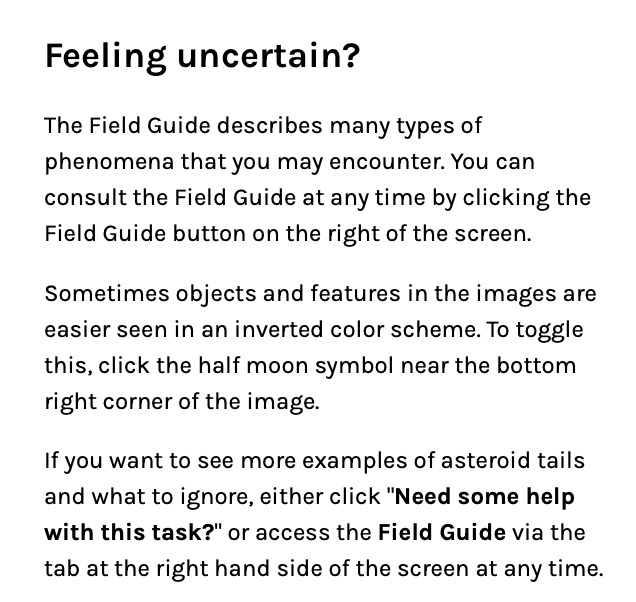} & \includegraphics[width=0.22\linewidth]{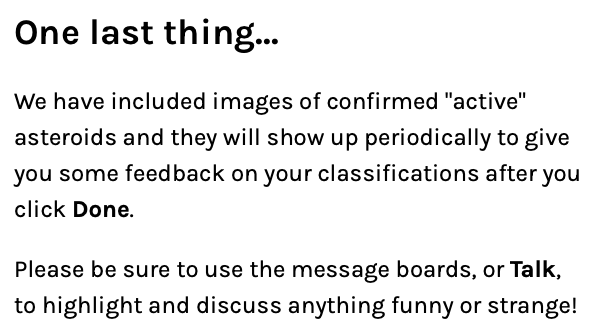} & \includegraphics[width=0.22\linewidth]{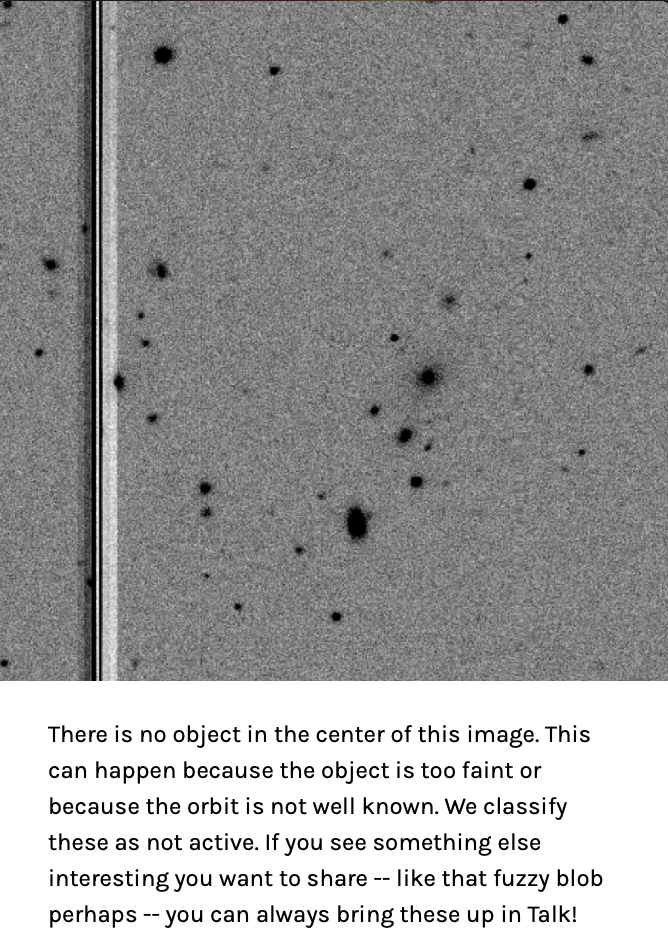}\\

        (5) & (6) & (7) & (8)\\

        % \hline\\

    \end{tabular}

    \caption{The \textit{Active Asteroids} Tutorial. (1) ``Welcome!'' provides a project overview. (2) ``Hot or Not?'' describes the workflow. (3) ``Tails'' describes tails with an example. (4) ``Comae'' introduces volunteers to the less familiar coma morphology. (5) ``Activity Look-a-Likes'' describes common false positive scenarios. (6) ``Feeling uncertain?'' explains what to do if a classification is ambiguous. (7) ``One last thing...'' lets users know about the injected training images. (8) This panel, requested by volunteers, describes a common situation where the object cannot be conclusively identified.}

    \label{methods:fig:tutorial}

\end{figure}

Figure \ref{methods:fig:tutorial} shows the eight panels of the project tutorial which is shown to volunteers the first time they participate in the project. The tutorial is also available at all times in a panel of the classification workflow window.

\subsection{Field Guide}

\label{sec:fieldGuideSupplemental}

\begin{itemize}

    \item \textbf{Asteroids (object of interest)} explains the object -- point source or trailed -- should be at center.

    \item \textbf{Trails (natural)} discusses trailed objects and rapid-rotators.

    \item \textbf{Tails (object of interest)} defines potential tail morphology and multiple tails.

    \item \textbf{Comae} describes comae and contrasts with tails.

    \item \textbf{Missing Object} acknowledges this scenario that we try to avoid (Section \ref{sec:sourceAnalysis}).

    \item \textbf{Crowded Fields} gives example fields containing many sources.

    \item \textbf{Blurry images} reiterates that these poor quality images should be skipped.

    \item \textbf{Galaxies} shows example galaxies, including active objects with background galaxies.

    \item \textbf{Cosmic Rays} defines the phenomenon and includes examples.

    \item \textbf{Trails (artificial)} briefly introduces (1) satellite trails and (2) telescope tracking issues.

    \item \textbf{Saturation and Scattered Light} explains how these phenomena could be mistaken for activity.

    \item \textbf{Background Object of Note (and size!)} gives interesting examples of clusters and dust clouds that take up a significant fraction of a thumbnail.

    \item \textbf{Donuts} describes out of focus images, with examples, including one with activity.

    \item \textbf{Dead Columns} provides examples of columnar artifacts intersecting the object of interest.

    \item \textbf{Partial Images (Edges and Corners)} supplies chip edge and corner examples.

    \item \textbf{Object width (object of interest)} discusses why sources appear to vary in width.

\end{itemize}
