# Supplementary material for: The Active Asteroids Citizen Science Program: Overview and First Results
Source: arXiv:2403.09768 source file (2024-03-14)
Supplement: Supplementary file 2 [file AppendixObjects.tex]

\section{Object Information}

\begin{table*}

\caption{Object Properties}

\label{tab:objectProperties}

\centering

\begin{tabular}{rlcccccrcrcrr}

\# & Name               & Class   & $N_\mathrm{act}$ & $q_\mathrm{last}$ & $q_\mathrm{next}$ & $T_\mathrm{J}$  & $a$     & $e$    & $i$    & $q$    & $Q$     & Period \\

 & & & & [UT] & [UT] & & [au] & & [deg] & [au] & [au] & yr\\

\hline

1  & Gault              & \acs{AA}      & 3    & 2023-07-04 & 2027-01-02 & 3.461 &  2.31  & 0.19 & 22.8 & 1.86 &  2.75  &  3.50   \\

2  & 2007 FZ$_{18}$     & \acs{AA*}     & 1    & 2018-03-07 & 2023-11-03 & 3.188 &  3.18  & 0.12 &  1.1 & 2.78 &  3.57  &  5.66   \\

3  & 2015 VA$_{108}$    & \acs{AA*}     & 1    & 2021-02-26 & 2026-09-11 & 3.160 &  3.13  & 0.22 &  8.5 & 2.45 &  3.81  &  5.54   \\

4  & 2010 LH$_{15}$     & \acs{MBC}     & 2    & 2019-09-09 & 2024-03-26 & 3.230 &  2.74  & 0.36 & 10.9 & 1.77 &  3.72  &  4.54   \\

5  & 2015 FW$_{412}$    & \acs{AA*}     & 1    & 2020-04-04 & 2024-11-08 & 3.280 &  2.76  & 0.16 & 13.7 & 2.32 &  3.21  &  4.60   \\

6  & 433P               & \acs{MBC}     & 2    & 2021-05-13 & 2026-09-23 & 3.193 &  3.06  & 0.23 &  0.1 & 2.37 &  3.75  &  5.37   \\

7  & C/2014 OG392       & Centaur       & 1    & 2021-12-09 & 2064-05-21 & 3.398 & 12.17  & 0.18 &  9.0 & 9.97 & 14.37  & 42.45   \\

8  & 282P               & \acs{QHC}     & 2    & 2021-10-24 & 2030-07-16 & 2.991 &  4.24  & 0.19 &  5.8 & 3.44 &  5.03  &  8.72   \\

9  & 2004 CV$_{50}$     & \acs{QHC}     & 1    & 2020-03-10 & 2025-08-28 & 3.061 &  3.10  & 0.44 &  1.4 & 1.73 &  4.48  &  5.47   \\

10 & 2009 DQ$_{118}$    & \acs{QHC}     & 1    & 2023-04-22 & 2030-01-26 & 3.004 &  3.58  & 0.32 &  9.4 & 2.43 &  4.72  &  6.76   \\

11 & 2018 CZ$_{16}$     & \acs{QHC}     & 1    & 2018-06-28 & 2024-11-26 & 2.995 &  3.45  & 0.34 & 13.7 & 2.27 &  4.63  &  6.41   \\

12 & 2019 OE$_{31}$     & \acs{QHC}     & 1    & 2019-07-22 & 2028-09-15 & 3.006 &  4.38  & 0.10 &  5.2 & 3.93 &  4.82  &  9.15   \\ % 9/25/2023 COC

13 & 2000 AU$_{242}$    & \acs{JFC}     & 1    & 2021-08-04 & 2032-02-11 & 2.738 &  4.80  & 0.49 &  9.5 & 2.46 &  7.14  & 10.52   \\

14 & 2005 XR$_{132}$    & \acs{JFC}     & 1    & 2020-11-26 & 2028-03-12 & 2.869 &  3.76  & 0.43 & 14.5 & 2.14 &  5.38  &  7.29   \\

15 & 2008 QZ$_{44}$     & \acs{JFC}     & 2    & 2017-03-23 & 2025-10-25 & 2.821 &  4.19  & 0.44 & 11.4 & 2.35 &  6.04  &  8.59   \\ % 9/25/2023 COC

16 & 2012 UQ$_{192}$    & \acs{JFC}     & 2    & 2020-08-10 & 2027-09-16 & 2.824 &  3.69  & 0.48 & 16.6 & 1.82 &  5.47  &  7.10   \\

17 & 2015 TC$_1$        & \acs{JFC}     & 1    & 2022-12-05 & 2030-04-06 & 2.789 &  3.77  & 0.49 & 17.8 & 1.91 &  5.64  &  7.33   \\

18 & 2017 QN$_{84}$     & \acs{JFC}     & 1    & 2017-08-08 & 2024-12-03 & 2.944 &  3.77  & 0.34 & 12.1 & 2.48 &  5.06  &  7.32   \\

19 & 2018 OR            & \acs{JFC}     & 1    & 2018-08-23 & 2025-04-16 & 2.861 &  3.53  & 0.54 &  2.1 & 1.64 &  5.43  &  6.65   \\

20 & 2018 VL$_{10}$     & \acs{JFC}     & 1    & 2018-12-31 & 2028-10-27 & 2.420 &  4.59  & 0.69 & 18.5 & 1.42 &  7.76  &  9.82   \\

\end{tabular}

\raggedright 

\\

Definitions: 

\acf{AA}, \acf{MBC}, \acs{AA}* is an \ac{MBC} candidate, \acf{JFC}, and \acf{QHC}. 

$N_\mathrm{act}$ number of activity epochs (separate orbits). 

$q_\mathrm{last}$, $q_\mathrm{next}$ last and next perihelion passage dates. 

$T_\mathrm{J}$ Tisserand parameter with respect to Jupiter. 

Semi-major axis $a$, eccentricity $e$, inclination $i$, $q$ and $Q$ the perihelion and aphelion distances.

\end{table*}

\section{Supplemental Images}% 8/10/2022 moving to pile-of-object format

\label{sec:supplementalimages}

Here we provide details about the individual objects discussed in this work. Objects are organized by dynamical class: active asteroids/\acfp{MBC}, active Centaurs, \acfp{QHA}, and \acfp{JFC}. Within each class, objects are ordered by provisional designation.% (and thus minor planet discovery order).

\subsection{Active Asteroids / Main-Belt Comets (MBCs)}\label{appendix:activeasteroids}

\label{appendix:Gault} % AA 9/15/2023 COC

\renewcommand{\thisobject}{(6478) Gault} % NOT checked JPL

\renewcommand{\thisfigsize}{0.23}

\begin{figure}

    \centering

    \begin{tabular}{cccc}

    	\labelpicA{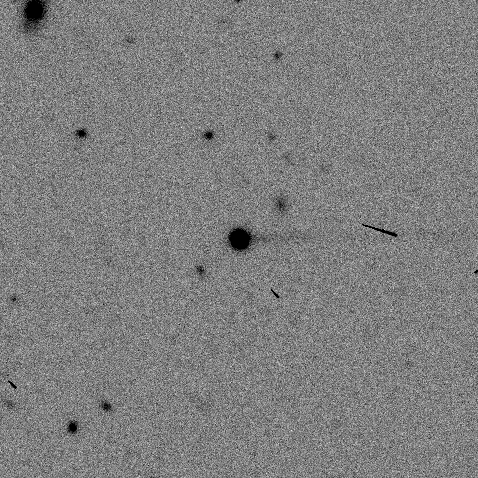}{a}{2013-09-28}{\thisfigsize}{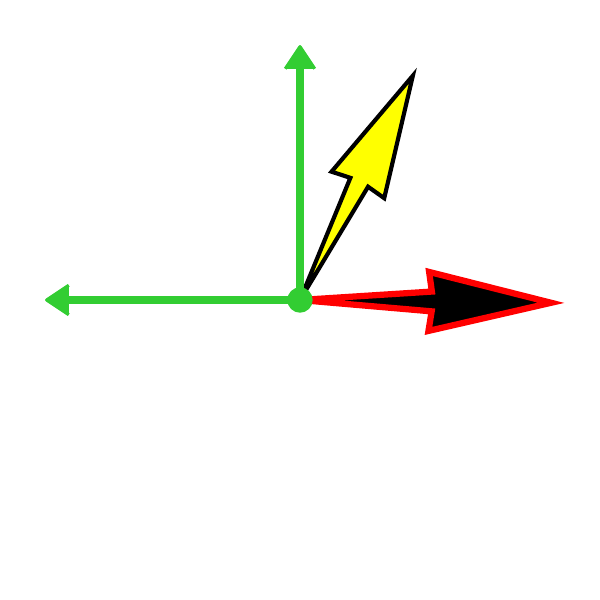} &

    \labelpicA{Gault_2016-06-09_04.46.31.479964_c4d_160609_044810_ooi_r_ls9_chip32-N2_126arcsec_NuEl.png}{b}{2016-06-09}{\thisfigsize}{Gault_2016-06-09_04.46.31.479964_c4d_160609_044810_ooi_r_ls9_chip32-N2_126arcsec_NuEl_arrows.pdf} &

    \labelpicA{Gault_2016-06-10_04.41.46.155704_c4d_160610_044331_ooi_g_ls9_chip32-N2_126arcsec_NuEl.png}{c}{2016-06-10}{\thisfigsize}{Gault_2016-06-10_04.41.46.155704_c4d_160610_044331_ooi_g_ls9_chip32-N2_126arcsec_NuEl_arrows.pdf}    &

	\labelpicA{Gault_2019-04-10_23.46.29.562427_c4d_190410_234549_ooi_g_ls10_chip15-S16_126arcsec_NuEl.png}{d}{2019-04-10}{\thisfigsize}{Gault_2019-04-10_23.46.29.562427_c4d_190410_234549_ooi_g_ls10_chip15-S16_126arcsec_NuEl_arrows.pdf}

    \end{tabular}

    \caption{\thisobject{}, at center, imaged by \ac{DECam}. The \acs{FOV} is 126''$\times$126'', with north up and east left. The projected anti-motion (red outlined black arrow) and anti-solar (yellow arrow) directions are shown.

    \textbf{(a)} UT 2013 September 28 90~s $g$ band (Prop. ID 2012B-0001, PI Frieman, observers SK, DT, NFM). This image appears in the gallery (Figure \ref{fig:galleryAll}a). 

    \textbf{(b)} UT 2016 June 9 96~s $r$ band (Prop. ID 2014B-0404, PI Schlegel, observer R. Blum). 

    \textbf{(c)} UT 2016 June 10 107~s $g$ band (Prop. ID 2014B-0404, PI Schlegel, observer R. Blum). 

    \textbf{(d)} UT 2019 April 10 80~s $g$ band (Prop. ID 2019A-0065, PI Shen, observer S. Malhotra). 

    }

    \label{fig:GaultAppendix}

    \label{fig:Gault:gallery}

\end{figure}

\label{appendix:2007FZ18} % MBC

\renewcommand{\thisobject}{(588045) 2007 FZ$_{18}$} % added number 3/15/2023 COC

\renewcommand{\thisfigsize}{0.35}

\begin{figure}

    \centering

 	\labelpicA{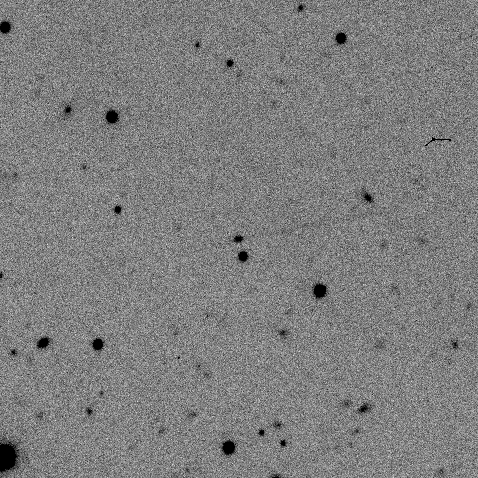}{}{}{0.25}{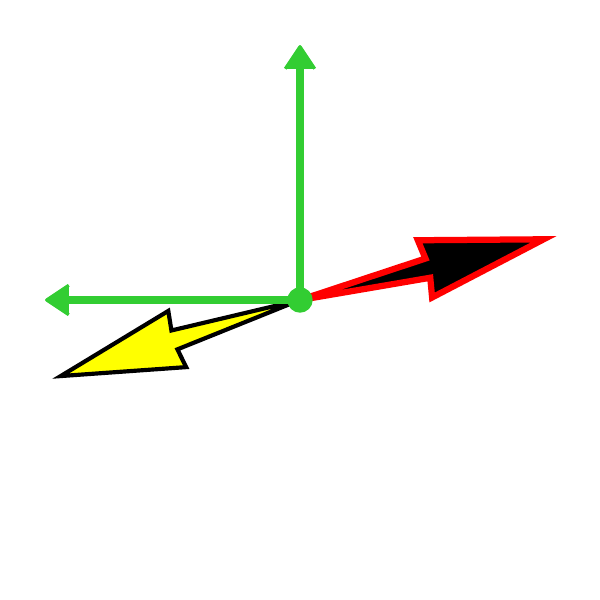}

    \caption{\thisobject{}, at the center, imaged by DECam on UT 2018 February 15 (Prop. ID 2014B-0404, PI Schlegel, observer S. Gontcho A Gontcho), with two tails: a long and thin tail in the anti-motion direction (red outlined black arrow), and a short faint tail in the anti-solar direction (yellow arrow), as projected on the sky. The FOV is 126''$\times$126'', with north up and east left. This image appears in the gallery (Figure \ref{fig:galleryAll}b).

    }

    \label{fig:2007FZ18}

    \label{fig:2007FZ18:gallery}

\end{figure}

\label{appendix:2010LH15} % MBC

\renewcommand{\thisobject}{2010 LH$_{15}$}

\renewcommand{\thisfigsize}{0.23}

\begin{figure}

    \centering

    \hspace{-13mm}

    \begin{tabular}{cccc}

        \labelpicA{2010_LH15_2010-09-27_11.45.36.869000_rings.v3.skycell.0970.085.wrp.i.55466_48935_chip1_126arcsec_NuEl.png}{a}{2010-09-27}{\thisfigsize}{2010_LH15_2010-09-27_11.45.36.869000_rings.v3.skycell.0970.085.wrp.i.55466_48935_chip1_126arcsec_NuEl_arrows.pdf} &

        \labelpicA{2010_LH15_2010-10-06_12.07.10.513000_rings.v3.skycell.0969.091.wrp.r.55475_50435_chip1_126arcsec_NuEl.png}{b}{2010-10-06}{\thisfigsize}{2010_LH15_2010-10-06_12.07.10.513000_rings.v3.skycell.0969.091.wrp.r.55475_50435_chip1_126arcsec_NuEl_arrows.pdf} & 

        \labelpicA{2010_LH15_2010-10-07_11.55.22.092000_rings.v3.skycell.1057.001.wrp.g.55476_49613_chip1_126arcsec_NuEl.png}{c}{2010-10-07}{\thisfigsize}{2010_LH15_2010-10-07_11.55.22.092000_rings.v3.skycell.1057.001.wrp.g.55476_49613_chip1_126arcsec_NuEl_arrows.pdf} &

        \labelpicA{2010_LH15_2010-12-08_07.17.09.130000_PTF_201012083032_i_p_scie_t071639_u010656646_f02_p110011_c02_chip0_126arcsec_NuEl.png}{d}{2010-12-08}{\thisfigsize}{2010_LH15_2010-12-08_07.17.09.130000_PTF_201012083032_i_p_scie_t071639_u010656646_f02_p110011_c02_chip0_126arcsec_NuEl_arrows.pdf}\\

        \labelpic{2010_LH15_2019-08-31_08.53.55.963000_ztf_20190831370440_000293_zr_c02_o_q4_sciimg_chip0-4_126arcsec_NuEl.png}{e}{2019-08-31}{\thisfigsize} &

        \labelpicA{2010_LH15_2019-09-30_02.35.59.092218_c4d_190930_023514_opi_i_v1_chip16-S17_126arcsec_NuEl.png}{f}{2019-09-30}{\thisfigsize}{2010_LH15_2019-09-30_02.35.59.092218_c4d_190930_023514_opi_i_v1_chip16-S17_126arcsec_NuEl_arrows.pdf}

    \end{tabular}

    % main gallery has rings.v3.skycell.0970.085.wrp.i.55466_47858

    \caption{\thisobject{} activity during two epochs: 2010 (top row) and 2019 (bottom row). 

    \textbf{(a)} UT 2010 September 27 Pan-STARRS 1 (1.8~m, Haleakala) 45~s $i$ band exposure. 

    \textbf{(b)} UT 2010 October 6 40~s $r$ band Pan-STARRS 1 (1.8~m, Haleakala) exposure. This image appears in the gallery (Figure \ref{fig:galleryAll}c). 

    \textbf{(c)} UT 2010 October 7 43~s $g$ band Pan-STARRS 1 (1.8~m, Haleakala) exposure. 

    \textbf{(d)} UT 2010 December 8 PTF (48'' Samuel Oschin telescope, Palomar) 60~s $i$ band exposure. 

    \textbf{(e)} UT 2019 August 31 30~s ZTF (48'' Samuel Oschin telescope, Palomar) $r$ band exposure. 

    \textbf{(f)} UT 2019 September 30 90~s exposure with DECam (Prop. ID 2019B-1014, PI Olivares, observers F. Olivares, I. Sanchez) on the Blanco 4~m telescope (CTIO, Chile). % Delve, Felipe Olivares, Ignacio Sanchez

    }

    \label{fig:2010LH15:gallery}

\end{figure}

\label{appendix:2015FW412} % MBC

\renewcommand{\thisobject}{2015 FW$_{412}$} % checked JPL 8/12/2022 COC

\renewcommand{\thisfigsize}{0.23}

\begin{figure}

    \centering

    \begin{tabular}{cccc}

	\labelpicA{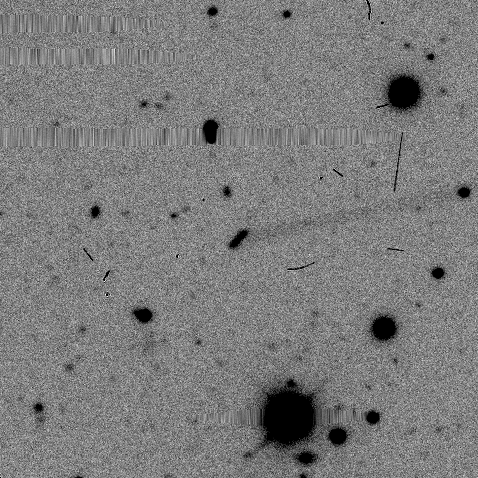}{a}{2015-04-13}{\thisfigsize}{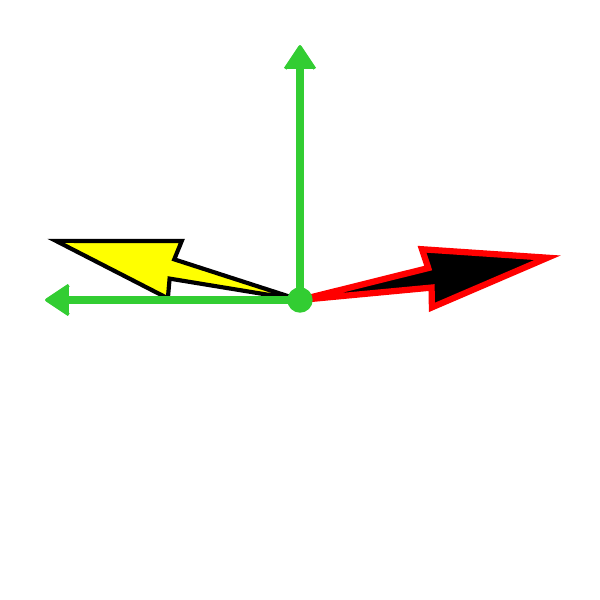}

        \labelpicA{2015_FW412_2015-04-18_02.22.54.528536_c4d_150418_022405_opi_VR_v1_chip52-N22_126arcsec_NuEl.png}{b}{2015-04-18}{\thisfigsize}{2015_FW412_2015-04-18_02.22.54.528536_c4d_150418_022405_opi_VR_v1_chip52-N22_126arcsec_NuEl_arrows.pdf} &

        \labelpicA{2015_FW412_2015-04-19_02.03.07.297521_c4d_150419_020417_opi_VR_v1_chip46-N16_126arcsec_NuEl.png}{c}{2015-04-19}{\thisfigsize}{2015_FW412_2015-04-19_02.03.07.297521_c4d_150419_020417_opi_VR_v1_chip46-N16_126arcsec_NuEl_arrows.pdf} &

        \labelpicA{2015_FW412_2015-04-22_02.05.09.421853_c4d_150422_020619_opi_VR_v1_chip19-S9_126arcsec_NuEl.png}{d}{2015-04-22}{\thisfigsize}{2015_FW412_2015-04-22_02.05.09.421853_c4d_150422_020619_opi_VR_v1_chip19-S9_126arcsec_NuEl_arrows.pdf} \\

    \end{tabular}

    \caption{\thisobject{} (at center) imaged with DECam in the \textit{VR} band filter, with a pronounced tail in the anti-motion (black arrow with red border) direction. Also indicated is the anti-solar direction (yellow arrow). 

    \textbf{(a)} UT 2015 April 13 360~s (Prop. ID 2015A-0351; PI Sheppard; observers S. Sheppard, C.Trujillo). This is the image included in the Gallery (Figure \ref{fig:galleryAll}d). 

    \textbf{(b)} UT 2015 April 18  40~s (Prop. ID 2013B-0536; PI Allen; observers L. Allen, D. James). 

    \textbf{(c)} UT 2015 April 19  40~s (Prop. ID 2013B-0536; PI Allen; observers L. Allen, D. James). 

    \textbf{(d)} UT 2015 April 22  40~s (Prop. ID 2013B-0536; PI Allen; observers L. Allen, D. James).

    }

    % c4d_150413_070257_opi is in the Gallery 8/29/2023 COC

    \label{fig:2015FW412:gallery}

\end{figure}

\label{appendix:2015VA108} % MBC

\renewcommand{\thisobject}{2015 VA$_{108}$}

\renewcommand{\thisfigsize}{0.23}

\begin{figure}

    \centering

    \begin{tabular}{cccc}

         \labelpicA{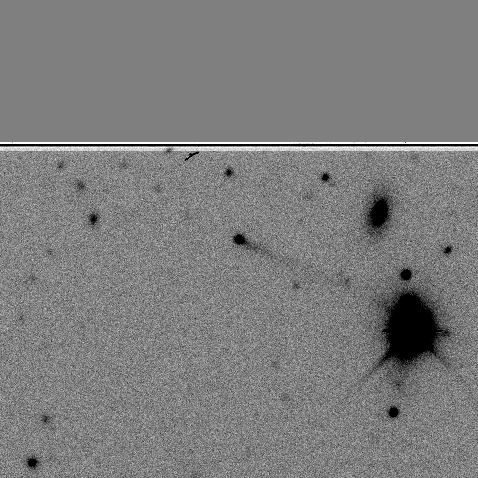}{a}{2015-10-11}{\thisfigsize}{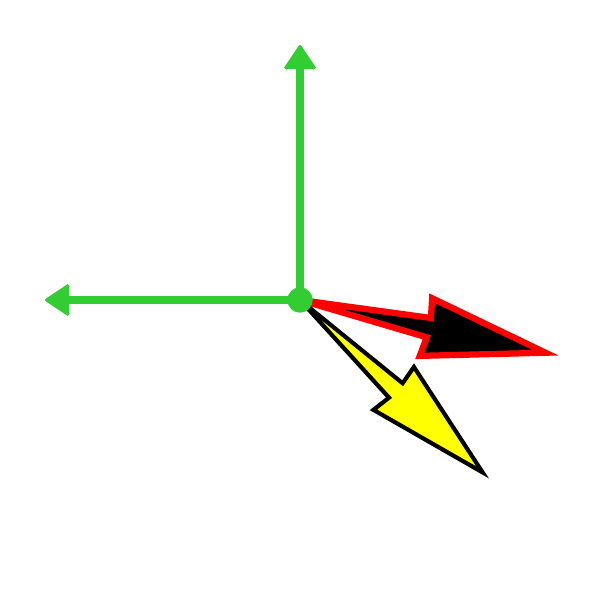} & \labelpicA{2015_VA108_2015-10-11_07.30.57.432576_c4d_151011_073251_ooi_g_ls9_chip36-N6_126arcsec_NuEl.png}{b}{2015-10-11}{\thisfigsize}{2015_VA108_2015-10-11_07.30.57.432576_c4d_151011_073251_ooi_g_ls9_chip36-N6_126arcsec_NuEl_arrows.pdf} &

    \end{tabular}

    % c4d_151011_073016_ooi is in the gallery

    \caption{\thisobject{} with a pronounced tail oriented between the anti-motion (black arrow with red border) and anti-solar (yellow arrow with black border) vectors as projected on sky. 

    % The FOV is 126''$\times$126'', with north up and east left. 

    Both images were acquired with \ac{DECam} on the Blanco 4~m telescope (Cerro Tololo Inter-American Observatory, Chile) on UT 2015 October 11 (Program 2014B-0404, PIs Schlegel and Dey, observers D. James, A. Dey, A. Patej). % David James, Arjun Dey, Anna Patej

    The FOV is roughly $126''\times 126''$, with north up and east left.  

    \textbf{(a)} 114~s $r$-band exposure. This image appears in the gallery (Figure \ref{fig:galleryAll}e). 

    \textbf{(b)} 125~s $g$-band exposure.

    }

    \label{fig:2015VA108:gallery}

\end{figure}

\label{appendix:433P} % MBC 9/15/2023 COC

\renewcommand{\thisobject}{(248370) 2005 QN$_{173}$} % NOT checked JPL

\renewcommand{\thisfigsize}{0.23}

\begin{figure}

    \centering

    \begin{tabular}{cccc}

    	\labelpicA{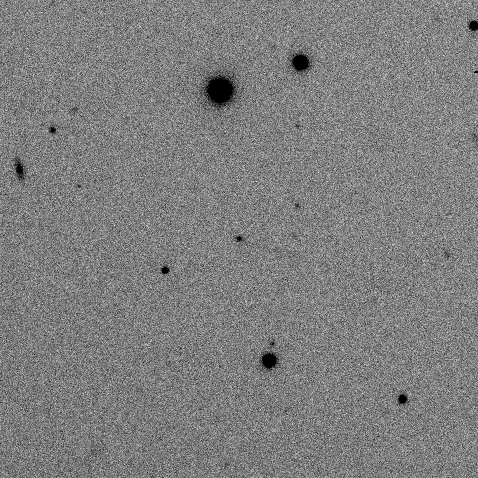}{a}{2016-07-22}{\thisfigsize}{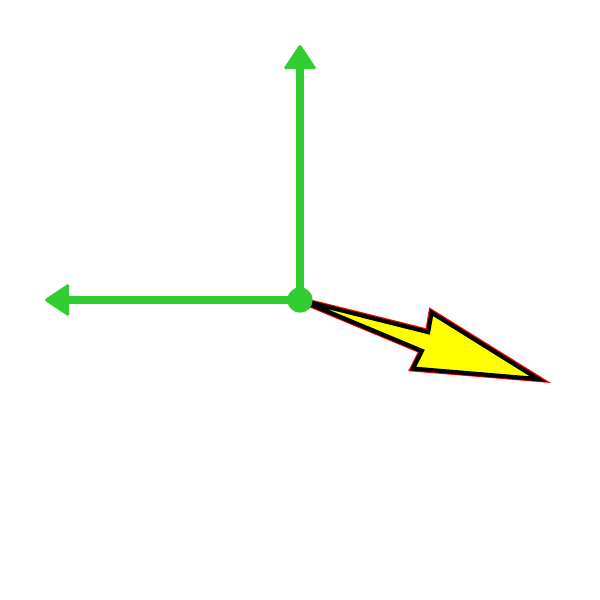} &

    	\labelpicA{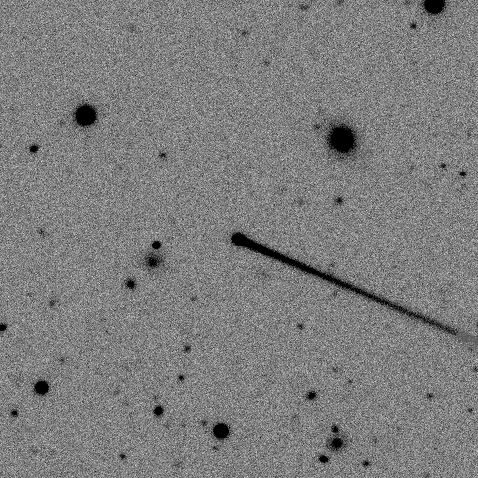}{b}{2019-09-03}{\thisfigsize}{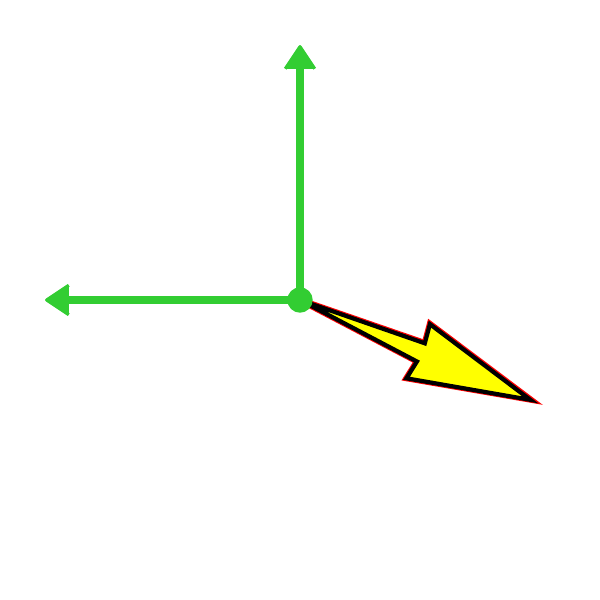}

    \end{tabular}

    \begin{tabular}{cc}

    \begin{overpic}[width=0.45\linewidth]{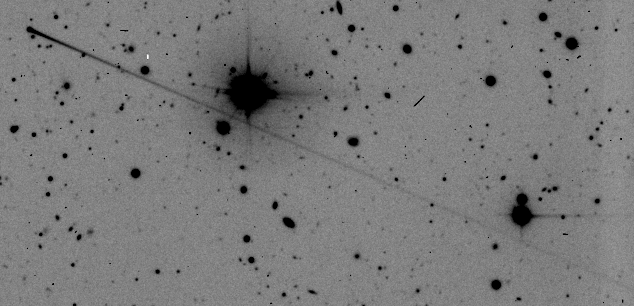}

	\put (5,6) {\huge\color{\labelcolor} \textbf{\contour{black}{c}}}

	\put (25,6) {\large\color{\labelcolor} \textbf{\contour{black}{2021-08-05}}}

\end{overpic} &

    \begin{overpic}[width=0.45\linewidth]{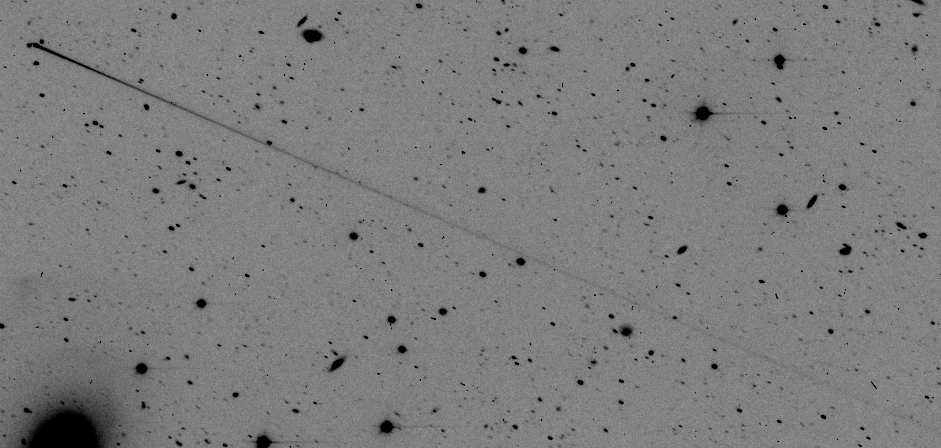}

	\put (5,6) {\huge\color{\labelcolor} \textbf{\contour{black}{d}}}

	\put (25,6) {\large\color{\labelcolor} \textbf{\contour{black}{2021-10-02}}}

\end{overpic}\\

\begin{overpic}[width=0.45\linewidth]{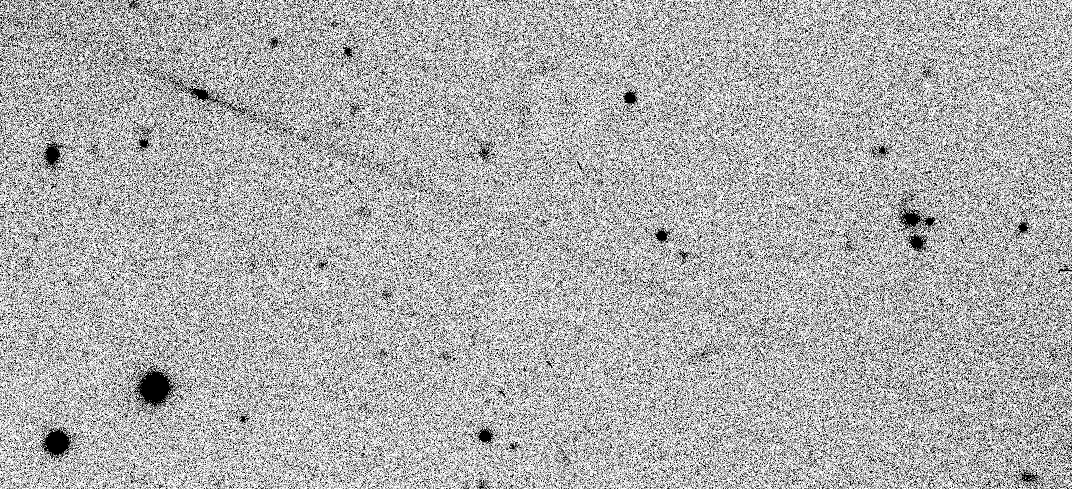}

	\put (5,6) {\huge\color{\labelcolor} \textbf{\contour{black}{e}}}

	\put (25,6) {\large\color{\labelcolor} \textbf{\contour{black}{2021-11-02}}}

\end{overpic} &

\begin{overpic}[width=0.45\linewidth]{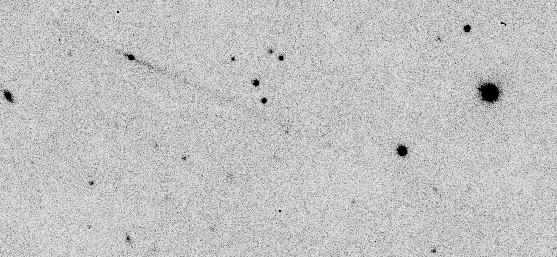}

	\put (5,6) {\huge\color{\labelcolor} \textbf{\contour{black}{f}}}

	\put (25,6) {\large\color{\labelcolor} \textbf{\contour{black}{2021-12-08}}}

\end{overpic}

    \end{tabular}

    \caption{\thisobject{}, at center in these 126\arcsec $\times$ 126\arcsec \acs{FOV} images acquired with \ac{DECam} asdf

     Indicated are the anti-motion direction (red outlined black arrow) and the anti-solar direction (yellow arrow), as projected on the sky. North is up and east left.

     \textbf{(a)} UT 2016 July 22 89~s $z$ band (Prop. ID 2016A-0190, PI Dey, observers D. Lang, A. Walker). % Dustin Lang, Alistair Walker

     This image appears in the gallery (Figure \ref{fig:galleryAll}f). 

     \textbf{(b)} UT 2021 September 3 60~s $r$ band (Prop. ID 2021B-0332, PI Shepparrd, observers S. Sheppard). 

     \textbf{(c)} UT 2021 August 5 \acf{LDT} \textit{VR} band exposure. %  TODO observers

     \textbf{(d)} UT 2021 October 2 \ac{LDT} \textit{r} band exposure. % TODO PI, observers.

     \textbf{(e)} UT 2021 November 2 \ac{LDT} 300~s filter exposure (PI Chandler, observers C. Chandler, C. Trujillo, W. Oldroyd).

     \textbf{(f)} UT 2021 December 8 \acf{VATT} exposure (PI Chandler, observers C. Chandler, W. Oldroyd.

     }

    \label{fig:433P}

    \label{fig:433P:gallery}

\end{figure}

The active asteroids (Section \ref{subsec:activeasteroids}) are 

(6478) Gault (Figure \ref{fig:Gault:gallery}), 

(588045) 2007 FZ18 (Figure \ref{fig:2007FZ18:gallery}), 

2010 LH$_{15}$ (Figure \ref{fig:2010LH15:gallery}),

2015 FW$_{412}$ (Figure \ref{fig:2015FW412:gallery}), 

2015 VA$_{108}$ (Figure \ref{fig:2015VA108:gallery}), 

and

433P (Figure \ref{fig:433P:gallery}).

\subsection{Active Centaurs}\label{appendix:centaurs}

\label{appendix:2014OG392}

\renewcommand{\thisobject}{C/2014 OG392 (PANSTARRS)} % 

\renewcommand{\thisfigsize}{0.23}

\begin{figure}

    \centering

    \begin{tabular}{cccc}

    	\labelpicA{C2014_OG392_2017-07-25_06.33.10.884783_c4d_170725_063434_ooi_r_ls9_chip14-S15_126arcsec_NuEl.png}{a}{2017-07-25}{\thisfigsize}{C2014_OG392_2017-07-25_06.33.10.884783_c4d_170725_063434_ooi_r_ls9_chip14-S15_126arcsec_NuEl_arrows.pdf} &

    	\labelpicA{C2014_OG392_2017-08-20_04.48.58.143889_c4d_170820_044824_ooi_r_ls9_chip42-N11_126arcsec_NuEl.png}{b}{}{\thisfigsize}{C2014_OG392_2017-08-20_04.48.58.143889_c4d_170820_044824_ooi_r_ls9_chip42-N11_126arcsec_NuEl_arrows.pdf} &

    	\labelpicA{C2014_OG392_2018-11-27_01.34.14.169017_c4d_181127_013329_ooi_g_ls9_chip35-N4_126arcsec_NuEl.png}{c}{}{\thisfigsize}{C2014_OG392_2018-11-27_01.34.14.169017_c4d_181127_013329_ooi_g_ls9_chip35-N4_126arcsec_NuEl_arrows.pdf} &

    	\labelpicA{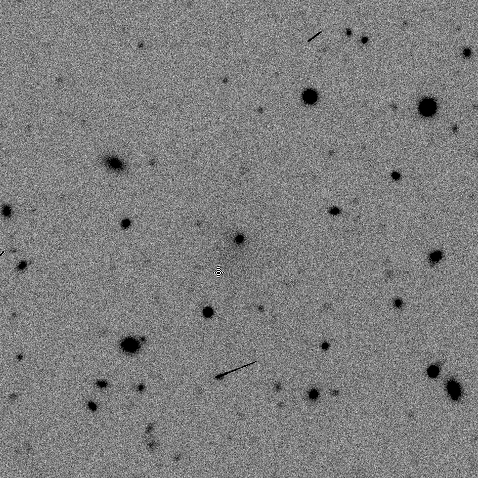}{d}{}{\thisfigsize}{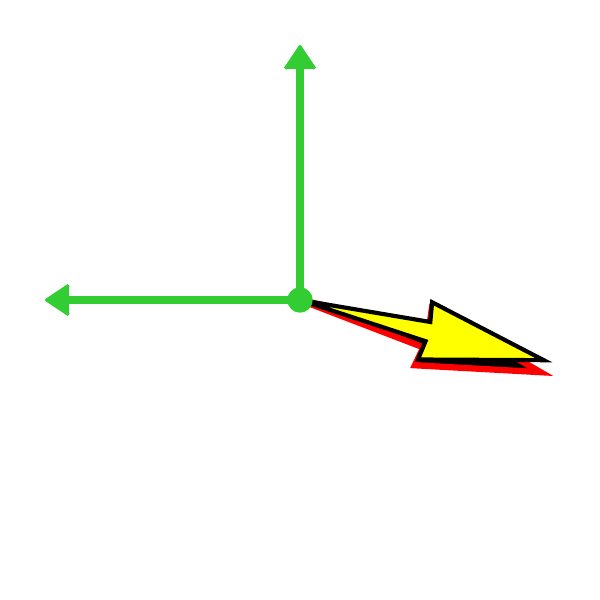}

    \end{tabular}

    \caption{\thisobject{}, at center in these 126\arcsec $\times$ 126\arcsec \acs{FOV} images acquired with \ac{DECam}. 

     Indicated are the anti-motion direction (red outlined black arrow) and the anti-solar direction (yellow arrow), as projected on the sky. North is up and east left.

     \textbf{(a)} UT 2017 July 25 52~s $r$ band (Prop. ID 2014B-0404, PI Schlegel, observer A. Walker). 

     \textbf{(b)} UT 2017 August 20 67~s $r$ band (Prop. ID 2014B-0404, PI Schlegel, observers T. Li, Y. Zhang). % Ting Li, Yuanyuan Zhang

     \textbf{(c)} UT 2018 November 27 90~s $g$ band (Prop. ID 2012B-0001, PI Frieman, observers R. Wilkinson, D. Turner, S. Bhargava). 

     \textbf{(d)} UT 2019 August 30 250~s \textit{VR} band (Prop. ID 2019A-0337, PI Trilling, observers C. Trujillo). This image appears in the gallery (Figure \ref{fig:galleryAll}g).

     }

    \label{fig:2014OG392}

    \label{fig:2014OG392:gallery}

\end{figure}

\subsection{Active Quasi-Hilda Asteroids (QHAs)}\label{appendix:qhas}

\label{subsec:282P} % known; QHC

\label{appendix:282P} % 9/11/2023 COC

\renewcommand{\thisobject}{282P/(323137) 2003 BM$_{80}$}

\renewcommand{\thisfigsize}{0.23}

\begin{figure}

    \centering

    \begin{tabular}{cccc}

         \labelpic{0323137H_20130505-06132_0733675_8.8y_qa_OC_150s_r-4_pI_ovX.png}{a}{2013-05-05}{\thisfigsize} & \labelpic{0323137H_20210314-08071_4179806_8.8y_qC_Ob_090s_i-3_p2_ovX.png}{b}{2021-03-14}{\thisfigsize} &

        \labelpic{0323137H_20210317-06133_4181183_8.8y_qC_Ob_090s_i-3_p2_ovX.png}{c}{2021-03-17}{\thisfigsize} & \labelpic{282P_20220607UT_GMOSS_MADS_gray_crop.png}{d}{2022-06-07}{\thisfigsize}

    \end{tabular}

    % c4d_210314_080717_opi appears in the gallery

    \caption{\thisobject{} images as shown to \textit{Active Asteroids} volunteers (a -- c), and an image (d) from our follow-up campaign. 

    \textbf{(a)} UT 2013 May 5 150~s $r$ band \ac{DECam} exposure Prop. (ID 2013A-0327, \acs{PI} Rest). A short tail is seen oriented towards around 7 o'clock. 

    \textbf{(b)} UT 2021 March 14 150~s $i$ band \ac{DECam} exposure (Prop. ID 2019A-0305 (\acs{PI} Drlica-Wagner). This image appears in the gallery (Figure \ref{fig:galleryAll}h). 

    \textbf{(c)} UT 2021 March 17 90~s $i$ band \ac{DECam} exposure (Prop. ID 2019A-0305 (\acs{PI} Drlica-Wagner). The right edge is the boundary of the CCD chip. 

    \textbf{(d)} UT 2022 June 7 coadded $6\times$ 120~s $g$-band Gemini South \acs{GMOS}-S images (Prop. ID GS-2022A-DD-103, \acs{PI} Chandler).

    }

    \label{fig:282P:gallery}

\end{figure}

\label{appendix:2004CV50} % QHC

\renewcommand{\thisobject}{2004 CV$_{50}$}

\renewcommand{\thisfigsize}{0.23}

\begin{figure}

    \centering

    \begin{tabular}{cccc}

         \labelpicA{2004_CV50_2020-02-15_08.48.22.758738_c4d_200215_084722_opi_i_v1_chip31-S7_126arcsec_NuEl.png}{a}{2020-02-15}{\thisfigsize}{2004_CV50_c4d_200215_084722_opi_i_v1_arrows.pdf} & 

         \labelpicA{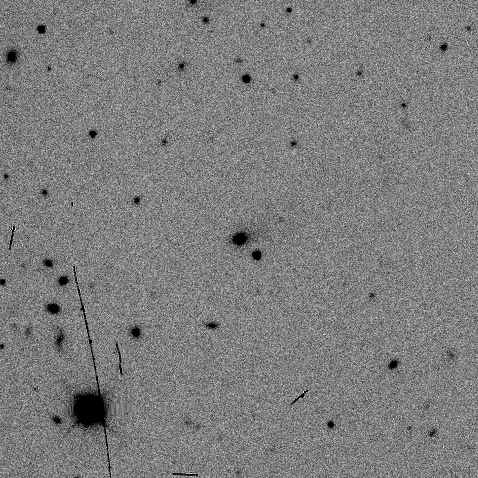}{b}{2020-03-14}{\thisfigsize}{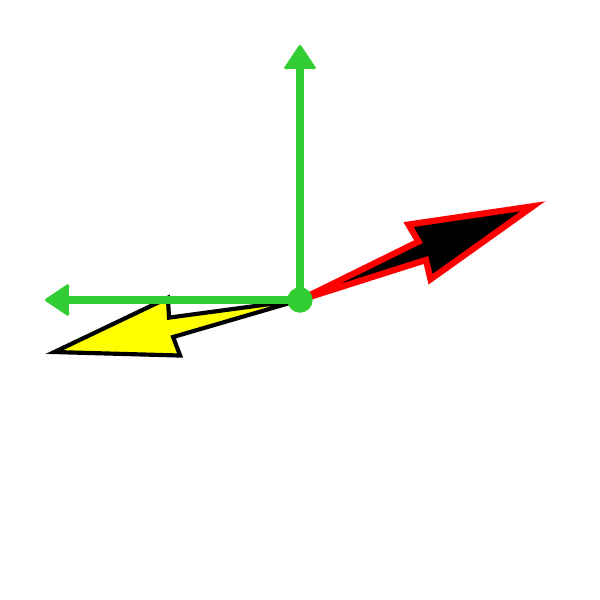} & 

         \labelpicA{2004_CV50_2020-03-14_06.46.22.579838_c4d_200314_064438_opi_i_v1_chip14-S15_126arcsec_NuEl.png}{c}{2020-03-14}{\thisfigsize}{2004_CV50_c4d_200314_064438_opi_i_v1_arrows.pdf} \\

    \end{tabular}

    % in gallery: 2004_CV50_2020-03-14_06.42.31.265554_c4d_200314_064053_opi_i_v1_chip3-S31_126arcsec_NuEl

    \caption{\thisobject{} (center) shows a diffuse tail towards the 2 o'clock direction in these 120~s $i$ band exposures taken with DECam on the Blanco 4~m telescope (\acs{CTIO}, Chile) by observer A. Diaz as part of the \acs{DECam} eROSITAS program (Prop. ID 2020A-0399; PI Zenteno). 

    The anti-motion (red outlined black arrow) and anti-solar (yellow arrow) directions, as projected on the sky, are marked. 

    The FOV is $126'' \times 126''$, with north up and east left. 

    \textbf{(a)} A diffuse tail is oriented towards the coincident anti-solar and anti-motion directions on UT 2020 February 15. The blank region is outside of the chip detector area. 

    \textbf{(b)} UT 2020 February 15. This image appears in the gallery (Figure \ref{fig:galleryAll}i). 

    \textbf{(c)} On UT 2020 March 14 a diffuse tail and coma are seen focused in the anti-motion direction.

    }

    \label{fig:2004CV50:gallery}

\end{figure}

\label{appendix:2009DQ118} % QHC 1/22/2023 COC/WJO

\renewcommand{\thisobject}{2009 DQ$_{118}$}

\renewcommand{\thisfigsize}{0.23}

\begin{figure}

    \centering

    \begin{tabular}{cccc}

        \labelpicA{2009_DQ118_2016-03-08_05.07.49.426225_c4d_160308_050956_opi_VR_v1_chip39-N9_126arcsec_NuEl.png}{a}{2016-03-08}{\thisfigsize}{2009_DQ118_2016-03-08_05.07.49.426225_c4d_160308_050956_opi_VR_v1_chip39-N9_126arcsec_NuEl_arrows.pdf} & 

	\labelpicA{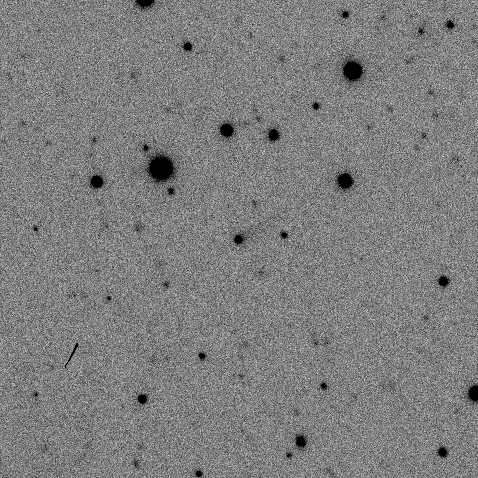}{b}{2016-03-09}{\thisfigsize}{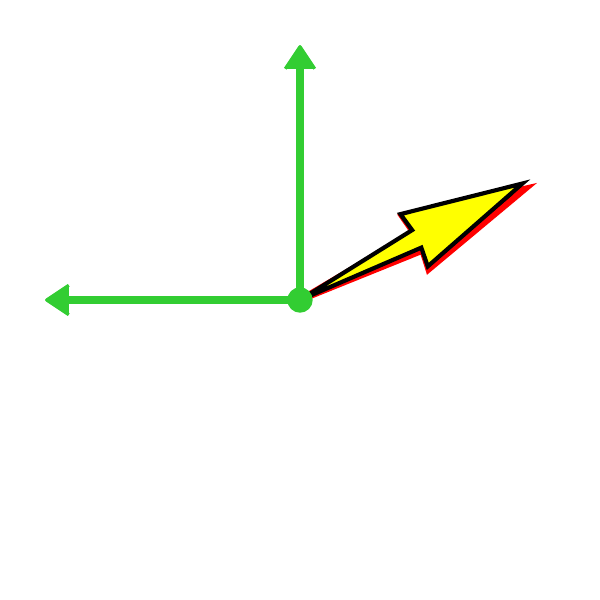} &

    % APO

    \labelpicA{2009_DQ118_2023-02-24_12.12.43.114546_red_image.0047.new_chip0_126arcsec_NuEl.png}{c}{2023-02-24}{\thisfigsize}{2009_DQ118_2023-02-24_12.12.43.114546_red_image.0047.new_chip0_126arcsec_NuEl_arrows.pdf} &

    \labelpicA{2009_DQ118_2023-04-22_05.20.14.900000_ift2047c2.new_chip0_126arcsec_NuEl.png}{d}{2023-04-22}{\thisfigsize}{2009_DQ118_2023-04-22_05.20.14.900000_ift2047c2.new_chip0_126arcsec_NuEl_arrows.pdf} % Magellan

    \end{tabular}

    % c4d_160309_070229_ooi is the gallery image 9/6/2023 COC changed

    \caption{\thisobject{}, at center, with a tail aligned roughly with the coincident anti-solar (yellow arrow) and anti-motion (red outlined black arrow) directions indicated. 

    The FOV is 126\arcsec$\times$ 126\arcsec with north up and east left. 

    \textbf{(a)} UT 2016 March 8 300~s \textit{VR} band \ac{DECam} exposure (Prop. ID 2016A-0189; PI Rest; observers A. Rest, DJJ). This image appears in the gallery (Figure \ref{fig:galleryAll}j). 

    \textbf{(b)} UT 2016 March 9 200~s $r$ band \ac{DECam} exposure (Prop. ID 2015A-0121; PI von der Linden; observer A. von der Linden).  % Anja von der Linden

    \textbf{(c)} UT 2023 February 24 300~s \textit{VR} band \ac{ARCTIC} exposure (program ID 2Q2023-UW08, PI Chandler, observers C. Chandler, W. Oldroyd.

    \textbf{(d)} UT 2023 April 22 150~s \textit{WB4800-7800} band \ac{IMACS} exposure (PI Sheppard, observer S. Sheppard).

    }

    \label{fig:2009DQ118:activity}

\end{figure}

\label{appendix:2018CZ16} % QHC; Chad lead

\renewcommand{\thisobject}{2018 CZ$_{16}$} % checked JPL 8/12/2022 COC

\renewcommand{\thisfigsize}{0.23}

\begin{figure}

    \centering

    \begin{tabular}{cccc}

       \labelpicA{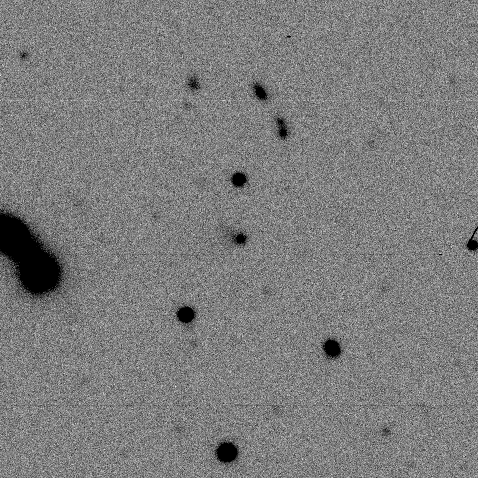}{a}{2018-05-15}{\thisfigsize}{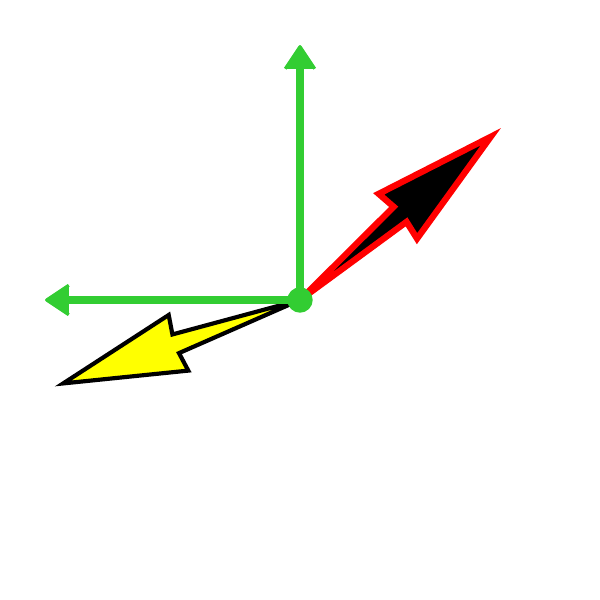} &

\labelpicA{2018_CZ16_2018-05-17_01.12.12.722517_c4d_180517_011127_ooi_g_ls9_chip51-N20_126arcsec_NuEl.png}{a}{2018-05-15}{\thisfigsize}{2018_CZ16_2018-05-17_01.12.12.722517_c4d_180517_011127_ooi_g_ls9_chip51-N20_126arcsec_NuEl_arrows.pdf} &

        \labelpicA{2018_CZ16_2018-05-17_23.17.25.666293_c4d_180517_231520_ooi_z_ls11_chip7-S28_126arcsec_NuEl.png}{b}{2018-05-17}{\thisfigsize}{2018_CZ16_2018-05-17_23.17.25.666293_c4d_180517_231520_ooi_z_ls11_chip7-S28_126arcsec_NuEl_arrows.pdf} &

        \labelpicA{2018_CZ16_2018-05-18_00.49.49.777056_c4d_180518_004809_ooi_g_ls9_chip7-S28_126arcsec_NuEl.png}{c}{2018-05-18}{\thisfigsize}{2018_CZ16_2018-05-18_00.49.49.777056_c4d_180518_004809_ooi_g_ls9_chip7-S28_126arcsec_NuEl_arrows.pdf}

        \\

    \end{tabular}

    % c4d_180515_004242_ooi is in the gallery

    \caption{\thisobject{} displays a faint tail oriented towards the anti-solar ($-\odot$) direction as projected on sky. Also indicated is the anti-motion direction ($-v$). All images were acquired with \acs{DECam} on the 4~m Blanco telescope (\acs{CTIO}, Chile) as part of Prop. ID 2014B-0404 (PI Schlegel). 

    \textbf{(a)} UT 2018 May 15 103~s $r$ band exposure. This image appears in the gallery (Figure \ref{fig:galleryAll}k).

    \textbf{(b)} UT 2018 May 17  90~s $g$ band image (observers E. Savary, A. Prakash). 

    \textbf{(c)} UT 2018 May 17 250~s $z$ band image (observer E. Savary). 

    \textbf{(d)} UT 2018 May 18 200~s $g$ band image (observer E. Savary). % Eloide Savary}

    }

    \label{fig:2018cz16:gallery}

\end{figure}

\subsection{2019 OE31} % added back 9/25/2023 COC

\label{appendix:2019OE31} % 9/25/2023 COC

\renewcommand{\thisobject}{2019 OE$_{31}$}

\begin{figure}[h]

    \centering

    \begin{tabular}{cccc}

    \labelpicA{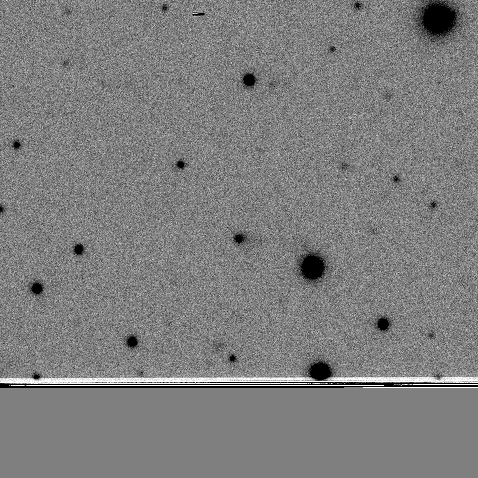}{}{2019-08-09}{0.31}{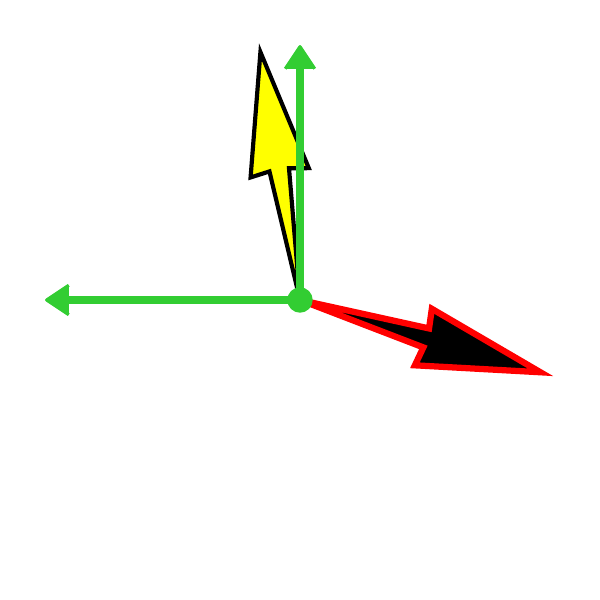}

    % \labelpicA{2019_OE31_2019-08-09_02.10.16.460122_c4d_190809_020931_opi_i_v1_chip48-N17_126arcsec_NuEl.png}{a}{2019-08-09}{2019_OE31_2019-08-09_02.10.16.460122_c4d_190809_020931_opi_i_v1_chip48-N17_126arcsec_NuEl_arrows.pdf}     &  

         \\

    \end{tabular}

    \caption{

    \thisobject{} (at center) in this 126\arcsec $\times$ 126\arcsec image (north is up and east is left). 

    The anti-solar (yellow arrow) and anti-motion (red outlined black arrow) directions, as projected on the sky, are marked. 

    On UT 2019 August 9 \thisobject{} displayed a diffuse tail oriented predominately towards the anti-motion direction. This 90~s $i$ band image was originally captured with DECam on UT 2019 August 9 (Prop. ID 2019A-0305; PI Drlica-Wagner; observers T. Li, K. Tavangar). 

    This image appears in the gallery (Figure \ref{fig:galleryAll}l).

    } % Ting Li, Kiyan Tavangar

    \label{fig:2019OE31:gallery}

\end{figure}

The active quasi-Hilda asteroids (QHAs), discussed in Section \ref{subsec:quasihildas}, are 

282P/(323137) 2003 BM$_{80}$ (Figure \ref{fig:282P:gallery}), 

2004 CV$_{50}$ (Figure \ref{fig:2004CV50:gallery}), 

2009 DQ$_{118}$ (Figure \ref{fig:2009DQ118:activity}), 

2018 CZ$_{16}$ (Figure \ref{fig:2018cz16:gallery}), 

and 

2019 OE$_{31}$ (Figure \ref{fig:2019OE31:gallery}).

\subsection{Jupiter Family Comets (JFCs)}\label{appendix:jfcs}

\label{appendix:2000AU242} % JFC

\renewcommand{\thisobject}{(275618) 2000 AU$_{242}$} % checked JPL 8/12/2022 COC

\renewcommand{\thisfigsize}{0.23}

\begin{figure}

    \centering

    \begin{tabular}{cccc}

        \labelpic{0275618T_20181113-05182_1526673_10.y_qs_Oa_107s_r-3_pI_ovX.png}{a}{2018-11-13}{\thisfigsize} & \labelpic{0275618T_20181113-05182_1526673_10.y_qs_Oa_107s_r-3_pI_ovX_POIMid778_c4d_180906_083638_ooi_g_v1.png}{b}{2018-11-13}{\thisfigsize}  \\

    \end{tabular}

    \caption{\thisobject{}. Two images of the same area of sky, acquired with \ac{DECam} on the Blanco 4~m telescope at (\acs{CTIO}, Chile) as part of \acs{NOAO} Prop. ID 2014B-0404 (\acs{PI} Schlegel). Here north is left and east is up. 

    \textbf{(a)} \thisobject{}, imaged UT 2018 November 13, in a 107~s $r$ band exposure. A tail is seen oriented towards the 10 o'clock position. This is the same instance as shown in the gallery (Figure \ref{fig:galleryAll}m). 

    \textbf{(b)} The same field as the left image, but at a time when \thisobject{} was not present. This 187~s $g$ band image from UT 2018 September 6 shows that there is no background source in this image that can account for the extended coma seen in the image at left.

    }

    \label{fig:2000AU242:gallery}

\end{figure}

\label{appendix:2005XR132} % JFC

\renewcommand{\thisobject}{2005 XR$_{132}$}

\renewcommand{\thisfigsize}{0.23}

\begin{figure}

    \centering

    \begin{tabular}{cccc}

        \hspace{-5mm}

		\labelpicA{2005_XR132_2021-02-08_11.36.11.075000_ztf_20210208483275_000270_zr_c06_o_q3_sciimg_chip0-3_126arcsec_NuEl.png}{a}{2021-02-08}{\thisfigsize}{2005_XR132_2021-02-08_11.36.11.075000_ztf_20210208483275_000270_zr_c06_o_q3_sciimg_chip0-3_126arcsec_NuEl_arrows.pdf} & 

		\labelpicA{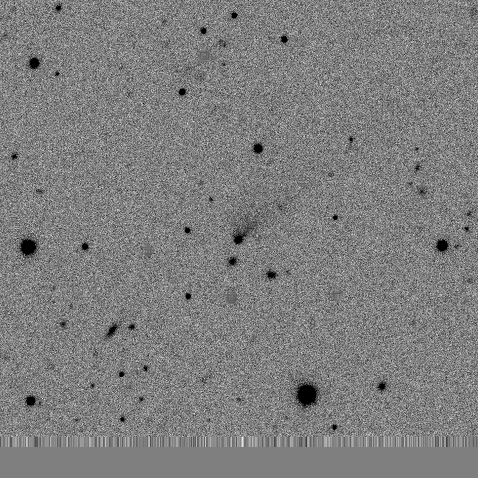}{b}{2021-03-26}{\thisfigsize}{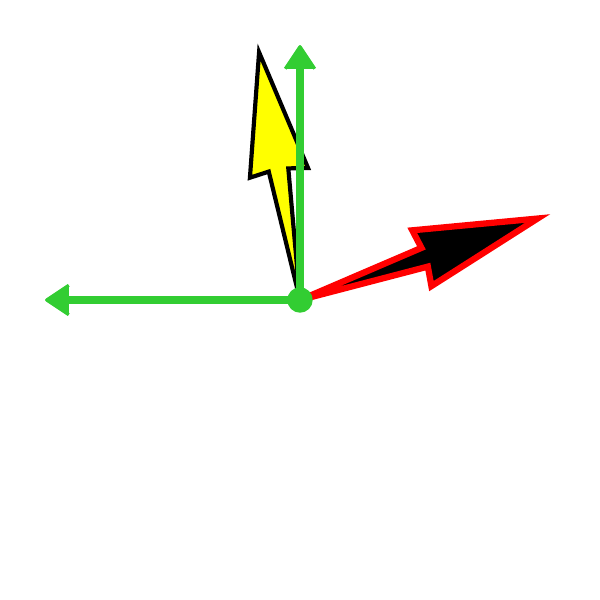}\\

    \end{tabular}

    % 210326_034047 appears in the gallery

    \caption{\thisobject{} (center) shows a tail spread between the anti-motion (red outlined black arrow) and anti-solar (yellow arrow) as projected on the sky. 

    The FOV is 126\arcsec$\times$ 126\arcsec. North is up and east is left. 

    \textbf{(a)} UT 2021 February 8 30~s $r$ band image acquired by \acs{ZTF} with the 48'' Samuel Oschin Telescope (Palomar Observatory, California). 

    \textbf{(b)} This 105~s $i$ band exposure was acquired UT 2021 March 26 with \acs{DECam} on the 4~m Blanco Telescope by observer A. Zenteno as part of the DeROSITAS program (Prop. ID 2021A-0149, PI Zenteno). This image appears in the gallery (Figure \ref{fig:galleryAll}n).

    }

    \label{fig:2005XR132}

    \label{fig:2005XR132:gallery}

\end{figure}

\label{appendix:2008_QZ44} % 9/25/2023 COC adding

\renewcommand{\thisobject}{2008 QZ$_{44}$} % 

\renewcommand{\thisfigsize}{0.23}

\begin{figure}

    \centering

    \begin{tabular}{cccc}

        \labelpicA{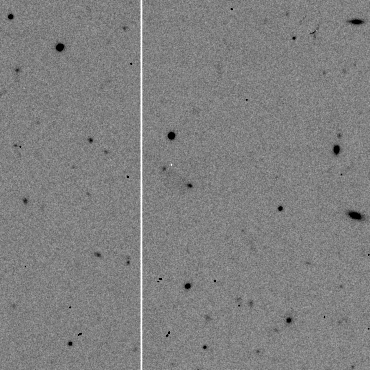}{a}{2008-11-20}{\thisfigsize}{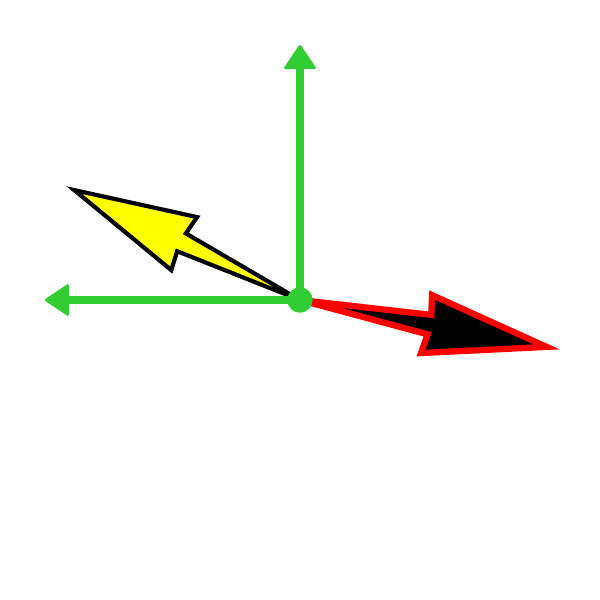} &

        \labelpicA{2008_QZ44_2017-11-12_04.49.16.799498_c4d_171112_044841_ooi_r_ls9_chip39-N8_126arcsec_NuEl.png}{b}{2017-11-12}{\thisfigsize}{2008_QZ44_2017-11-12_04.49.16.799498_c4d_171112_044841_ooi_r_ls9_chip39-N8_126arcsec_NuEl_arrows.pdf}

    \end{tabular}

    \caption{\thisobject{}, at center in these 126\arcsec $\times$ 126\arcsec \acs{FOV} \ac{DECam} images. 

     Indicated are the anti-motion direction (red outlined black arrow) and the anti-solar direction (yellow arrow), as projected on the sky. North is up and east left.

     \textbf{(a)} UT 2008 November 20 120~s \textit{g}-band MegaPrime image acquired with the \ac{CFHT} on Mauna Kea, Hawaii (PI Hoekstra, observers ``QSO Team''). A tail is seen oriented towards the anti-solar direction. This image is in the gallery (Figure \ref{fig:galleryAll}o). 

    \textbf{(b)} UT 2017 November 12 71~s \textit{r}-band image acquired with \ac{DECam} (prop. ID ID 2014B-0404, PI Schlegel, observers C. Stillman, J. Moustakas, M. Poemba). A faint tail is oriented towards the 2 o'clock position, between the anti-solar and anti-motion vectors.

     }

    \label{fig:2008QZ44}

    \label{fig:2008QZ44:gallery}

\end{figure}

\label{appendix:2012UQ192} % JFC

\renewcommand{\thisobject}{(551023) 2012 UQ$_{192}$} % checked JPL 8/11/2022 COC

\renewcommand{\thisfigsize}{0.23}

\begin{figure}

    \centering

    \begin{tabular}{cccc}

	\labelpicA{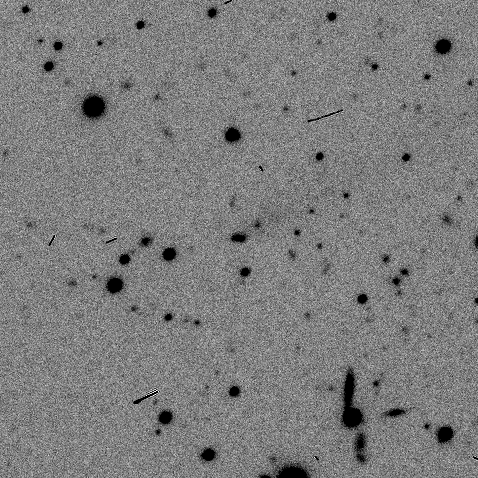}{a}{2014-04-30}{\thisfigsize}{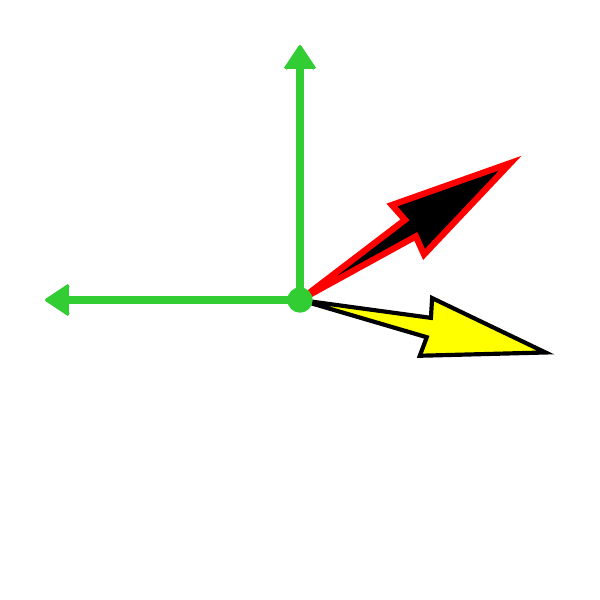}

        & \labelpicA{0935213A_20140505-05435_0881685_7.1y_qI_Oa_300s_T-4_pI_ovX.png}{b}{2014-05-05}{\thisfigsize}{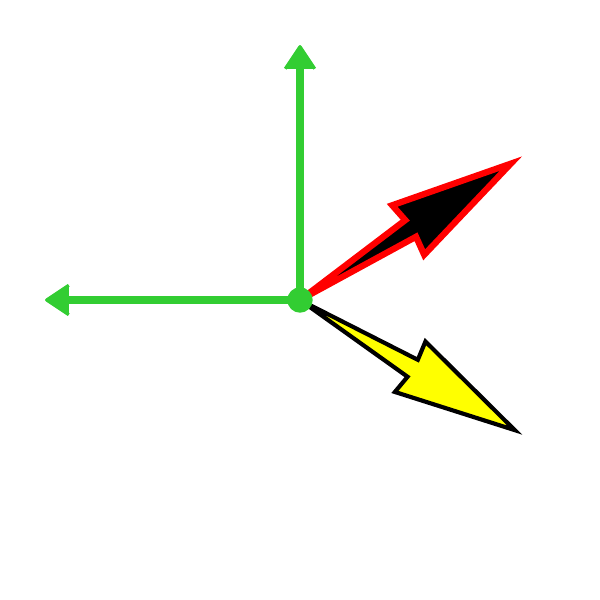} & % special arrows because archive file now missing from AstroArchive(!?) 9/11/2023 COC

        \labelpicA{2012_UQ192_2020-11-24_12.59.39.033000_ztf_20201124541238_000475_zr_c10_o_q3_sciimg_chip0-3_126arcsec_NuEl.png}{c}{2020-11-24}{\thisfigsize}{2012_UQ192_2020-11-24_12.59.39.033000_ztf_20201124541238_000475_zr_c10_o_q3_sciimg_chip0-3_126arcsec_NuEl_arrows.pdf}

        & \labelpicA{2012_UQ192_2021-01-17_11.56.06.822000_ztf_20210117497095_000427_zr_c07_o_q1_sciimg_chip0-1_126arcsec_NuEl.png}{d}{2021-01-17}{\thisfigsize}{2012_UQ192_2021-01-17_11.56.06.822000_ztf_20210117497095_000427_zr_c07_o_q1_sciimg_chip0-1_126arcsec_NuEl_arrows.pdf}\\

    \end{tabular}

    \caption{\thisobject{} displays a tail during two activity epochs. The anti-motion (black arrow with red border) and anti-solar (yellow arrow) directions as projected on sky are indicated. 

    The FOV is $126'' \times 126''$, with north up and east left. 

    All 2015 images were 300~s VR band exposures, originally acquired with \acs{DECam} on the 4~m Blanco telescope (\acs{CTIO}, Chile) as part of Prop. ID 2014A-0283 (PI: Trilling) with observers D. Trilling and L. Allen (both dates) plus J. Rajagopal (April 30) and T. Axelrod (May 5). 

    The 2020 -- 2021 images were acquired with the \acs{ZTF} camera on the 48'' Samuel Oschin Telescope (Palomar Observatory, California). 

    \textbf{(a)} UT 2014 April 30 exposure. This image appears in the gallery (Figure \ref{fig:galleryAll}p). 

    \textbf{(b)} Image from UT 2014 May 5. 

    \textbf{(c)} Six co-added 30~s $r$ band images from UT 2020 November 24 -- 26. 

    \textbf{(d)} UT 2021 January 17 30~s $r$ band exposure.

    }

    \label{fig:2012uq192:gallery}

\end{figure}

\label{appendix:2015TC1}

\renewcommand{\thisobject}{2015 TC$_{1}$} % checked JPL 8/12/2022 COC

\renewcommand{\thisfigsize}{0.23}

\begin{figure}

    \centering

    \begin{tabular}{cccc}

        \labelpicA{2015_TC1_2015-10-07_05.25.58.682445_c4d_151007_052734_ooi_r_ls9_chip46-N16_126arcsec_NuEl.png}{a}{2015-10-07}{\thisfigsize}{2015_TC1_2015-10-07_05.25.58.682445_c4d_151007_052734_ooi_r_ls9_chip46-N16_126arcsec_NuEl_arrows.pdf} & 

        \labelpicA{2015_TC1_2015-10-08_04.48.23.605950_c4d_151008_044956_ooi_g_ls9_chip28-S5_126arcsec_NuEl.png}{b}{2015-10-08}{\thisfigsize}{2015_TC1_2015-10-08_04.48.23.605950_c4d_151008_044956_ooi_g_ls9_chip28-S5_126arcsec_NuEl_arrows.pdf} &

         \labelpicA{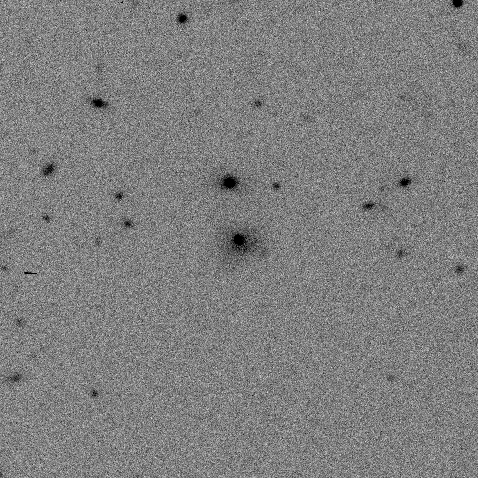}{c}{2015-12-19}{\thisfigsize}{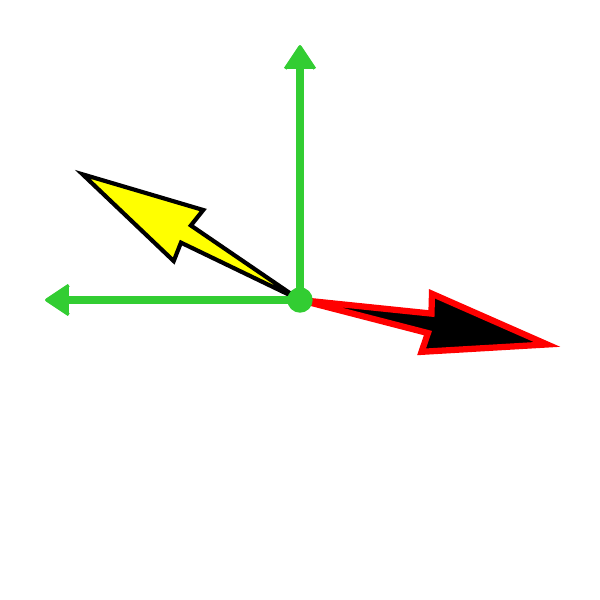} &

         \labelpicA{2015_TC1_2016-01-01_01.30.19.055804_c4d_160101_013154_ooi_g_ls9_chip55-N25_126arcsec_NuEl.png}{d}{2016-01-01}{\thisfigsize}{2015_TC1_2016-01-01_01.30.19.055804_c4d_160101_013154_ooi_g_ls9_chip55-N25_126arcsec_NuEl_arrows.pdf}

    \end{tabular}

    % c4d_151219_025516_ooi appears in the gallery

    \caption{\thisobject{}. Activity in 90~s images acquired with \ac{DECam} on the Blanco 4~m telescope at the \ac{CTIO} in Chile. All images were acquired as part of proposal ID 2012B-0001, PI Frieman. 

    \textbf{(a)} UT 2015 October 5 $r$ band exposure (observers S. S. Tie, B. Nord, D. Tucker). %Suk Sien Tie, B. Nord, D. Tucker

    \textbf{(b)} UT 2015 October 10 $g$ band exposure (observers S.S. Tie, T. Abbott, C. Furlanetto). 

    \textbf{(c)} UT 2015 December 19 $z$ band exposure (observers J. Allyn Smith, E. Balbinot). This image appears in the gallery (Figure \ref{fig:galleryAll}q). 

    \textbf{(d)} UT 2016 January 1 $g$ band exposure (observers D. Gerdes, S. Jouvel).

    }

    \label{fig:2015TC1:gallery}

\end{figure}

\label{appendix:2017QN84} % JFC

\renewcommand{\thisobject}{2017 QN$_{84}$} % checked JPL 8/12/2022 COC

\renewcommand{\thisfigsize}{0.23}

\begin{figure}

    \centering

    \begin{tabular}{cccc}

        \labelpicA{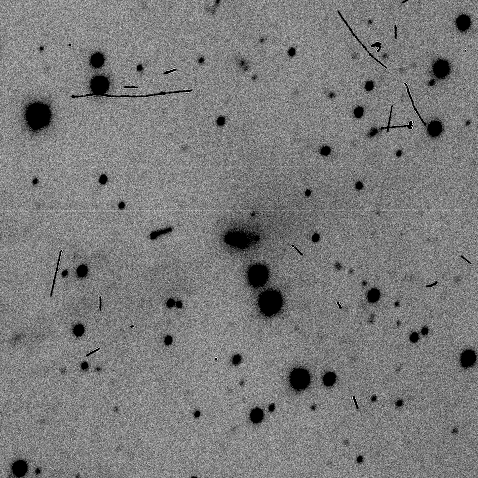}{a}{2017-12-23}{\thisfigsize}{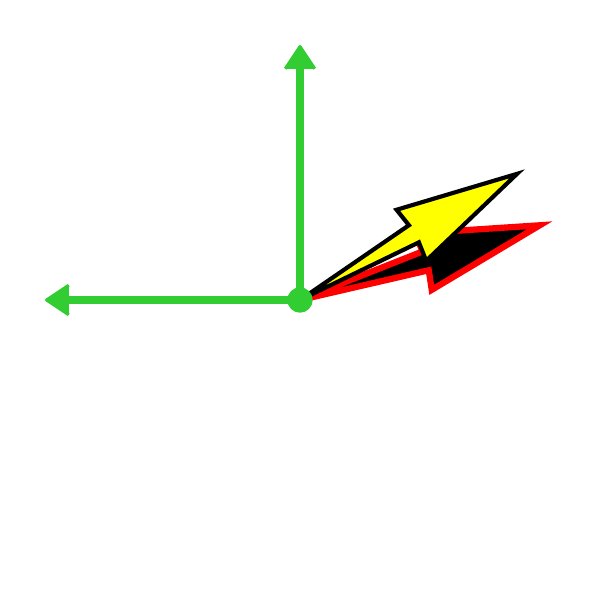} & 

        \labelpic{0888084H_20171223-07553_1283382_7.3y_qb_OC_600s_r-5_pI_ovX_POIMid29_2017-12-24_07.35.46_c4d_171224_073046_ooi_r_v1_chip2-S30_240pix_NuElnoArrows.png}{b}{2017-12-24}{\thisfigsize} \\

    \end{tabular}

    \caption{\thisobject{}. Two 600~s $r$ band \ac{DECam} images (Prop. ID 2017B-0307, \acs{PI} Sheppard) of the same field. 

    \textbf{(a)} \thisobject{}, imaged on UT 2017 December 23. The same instance appears in the gallery (Figure \ref{fig:galleryAll}r). 

    \textbf{(b)} This comparison \ac{DECam} image from UT 2017 December 24 shows the same field of view as the image at left with comparable depth, but this image was acquired when \thisobject{} was not in the \acs{FOV}.

    }

    \label{fig:2017qn84}

    \label{fig:2017qn84:gallery}

\end{figure}

\label{appendix:2018OR} % JFC/Mars-Crosser, KAF lead

\renewcommand{\thisobject}{2018 OR} % checked JPL 8/12/2022 COC

\renewcommand{\thisfigsize}{0.23}

\begin{figure}

    \centering

    \begin{tabular}{cccc}

        \labelpicA{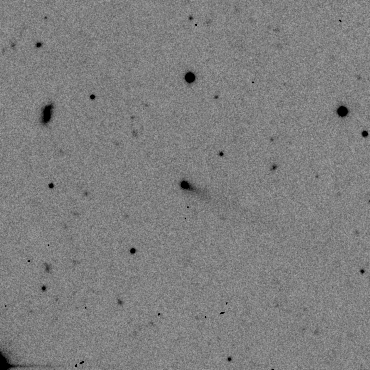}{a}{2018-09-05}{\thisfigsize}{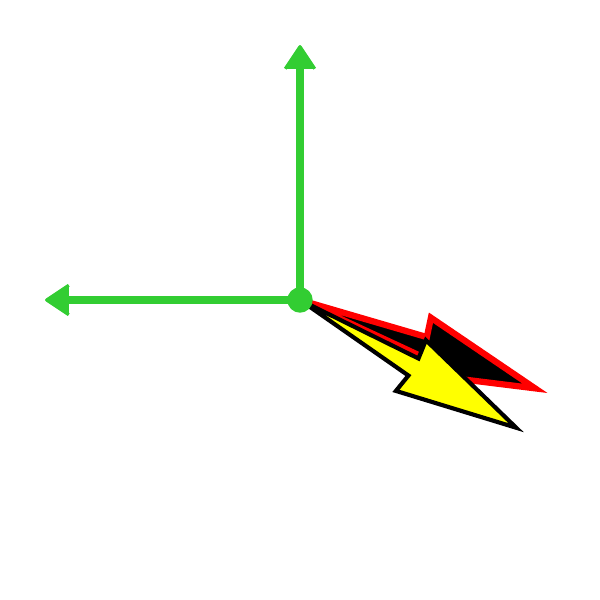} &

        \labelpicA{2018_OR_2018-09-06_03.38.06.645735_c4d_180906_033743_ooi_r_ls9_chip37-N6_126arcsec_NuEl.png}{b}{2018-09-06}{\thisfigsize}{2018_OR_2018-09-06_03.36.21.531997_c4d_180906_033528_ooi_g_ls9_chip37-N6_126arcsec_NuEl_arrows.pdf} &

        \labelpicA{2018_OR_2018-09-17_09.15.34.084000_ztf_20180917385613_000448_zr_c16_o_q2_sciimg_chip0-2_126arcsec_NuEl.png}{c}{2018-09-17}{\thisfigsize}{2018_OR_2018-09-17_09.15.34.084000_ztf_20180917385613_000448_zr_c16_o_q2_sciimg_chip0-2_126arcsec_NuEl_arrows.pdf} &

        \labelpicA{2018_OR_2018-09-18_03.07.00.839206_c4d_180918_030610_ooi_z_ls9_chip48-N17_126arcsec_NuEl.png}{d}{2018-09-18}{\thisfigsize}{2018_OR_2018-09-18_03.07.00.839206_c4d_180918_030610_ooi_z_ls9_chip48-N17_126arcsec_NuEl_arrows.pdf}

    \end{tabular}

    % 018_OR_2018-09-05_11.11.27.292000_2300313p_chip24-ccd23 is in the gallery

    \caption{\thisobject{} at center in four 126\arcsec $\times$ 126\arcsec \ac{FOV} images. When provided, red -$v$ and yellow -$\odot$ indicate the anti-motion and anti-solar vectors, respectively. \acs{DECam} was on the 4~m Blanco telescope (\acs{CTIO}, Chile). 

    \textbf{(a)} 60~s \textit{GRI} band image from UT 2018 September 5 (Prop. ID 18BH09, \acs{PI} Wainscoat) with MegaPrime on the \ac{CFHT}. This image appears in the gallery (Figure \ref{fig:galleryAll}s). 

    \textbf{(b)} This 46~s $r$ \ac{DECam} image, acquired UT 2018 September 6 (Prop. ID 2014B-0404, \acs{PI} Schlegel) was classified as active by % [TODO@WAB]\% of 

    volunteers of the \textit{Active Asteroids} Citizen Science project. 

    \textbf{(c)} A 30~s $r$ band image acquired UT 2018 September 17 as part of the \ac{ZTF} survey with the \acs{ZTF} camera on the 48'' Samual Oschin telescope (Palomar Observatory, California). % TODO acknowledge, cite, etc. as needed

    \textbf{(d)} 100~s $z$ band \ac{DECam} image from UT 2018 September 18 (Prop. ID 2014B-0404, \acs{PI} Schlegel).

    }

    \label{fig:2018or:gallery}

\end{figure}

\label{appendix:2018VL10} % JFC

\renewcommand{\thisobject}{2018 VL$_{10}$} % checked JPL 8/12/2022 COC

\renewcommand{\thisfigsize}{0.23}

\begin{figure}

    \centering

    \begin{tabular}{cccc}

    	\labelpicA{2018_VL10_2018-12-31_05.17.04.865909_c4d_181231_051549_opi_VR_v1_chip14-S15_126arcsec_NuEl.png}{a}{2018-12-31}{\thisfigsize}{2018_VL10_2018-12-31_05.17.04.865909_c4d_181231_051549_opi_VR_v1_chip14-S15_126arcsec_NuEl_arrows.pdf} & 

     \labelpicA{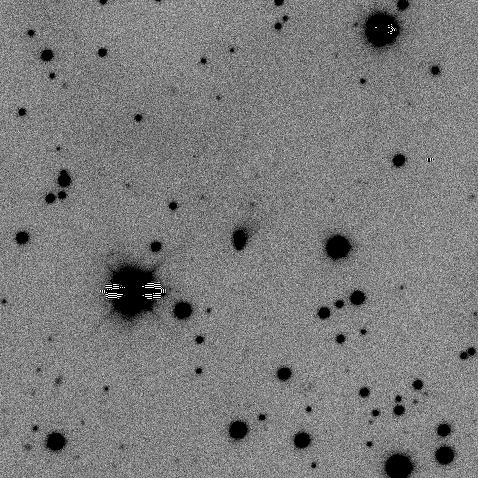}{b}{2018-12-31}{\thisfigsize}{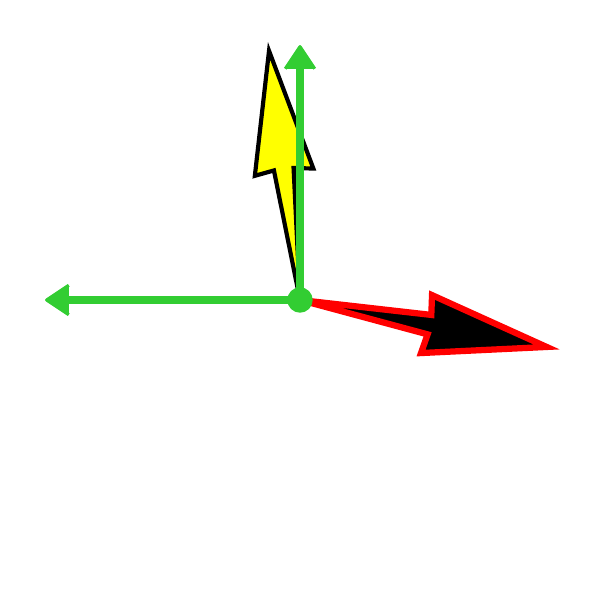} &

    \labelpicA{2018_VL10_2019-02-01_03.57.52.337103_c4d_190201_035637_opi_VR_v1_chip58-N27_126arcsec_NuEl.png}{c}{2019-02-01}{\thisfigsize}{2018_VL10_2019-02-01_03.57.52.337103_c4d_190201_035637_opi_VR_v1_chip58-N27_126arcsec_NuEl_arrows.pdf} & 

    \labelpicA{2018_VL10_2019-02-01_04.00.50.875420_c4d_190201_035935_opi_VR_v1_chip58-N27_126arcsec_NuEl.png}{d}{2019-02-01}{\thisfigsize}{2018_VL10_2019-02-01_04.00.50.875420_c4d_190201_035935_opi_VR_v1_chip58-N27_126arcsec_NuEl_arrows.pdf}\\

    \end{tabular}

    % c4d_181231_051849_opi is in the gallery

    \caption{\thisobject{} (at center) displays activity in these pairs of 150~s $VR$ band images acquired with \acs{DECam} on the 4~m Blanco telescope (\acs{CTIO}, Chile) as part of Prop. ID 2018B-0122 (PI Rest). 

    \textbf{(a)} and \textbf{(b)}: UT 2018 December 31 (observer A. Zenteno). (b) appears in the gallery (Figure \ref{fig:galleryAll}t). 

    \textbf{(c)} and \textbf{d}: UT 2019 February 1 (observers A. Rest, A. Zenteno).  % Armin Rest, Alfredo Zenteno

    }

    \label{fig:2018vl10:gallery}

\end{figure}

The Jupiter Family Comets (Section \ref{subsec:jfcs}) included here are 

(275618) 2000 AU$_{242}$ (Figure \ref{fig:2000AU242:gallery}), 

2005 XR$_{132}$ (Figure \ref{fig:2005XR132:gallery}), 

(551023) 2012 UQ$_{192}$ (Figure \ref{fig:2012uq192:gallery}), 

2008 QZ$_{44}$ (Figure \ref{fig:2008QZ44:gallery}), 

2015 TC$_1$ (Figure \ref{fig:2015TC1:gallery}), 

2017 QN$_{84}$ (Figure \ref{fig:2017qn84:gallery}), 

2018 OR (Figure \ref{fig:2018or:gallery}), 

and 

2018 VL$_{10}$ (Figure \ref{fig:2018vl10:gallery}).
